# Supplementary material for: Anisotropic marginal Fermi liquid for Coulomb interacting generalized Weyl fermions
Source: arXiv:2602.17666 ancillary file (2026-06-08)
Supplement: Supplementary file 1 [file SM.pdf]

# Supplementary Materials: Anisotropic marginal Fermi liquid for Coulomb interacting generalized Weyl fermions


Gabriel Malavé[1,2], Rodrigo Soto-Garrido[2], Bitan Roy[3], and Vladimir Juričić[4]

[1]Department of Physics and Astronomy, Rutgers University, Piscataway, NJ 08854, USA
[2]Instituto de Física, Pontificia Universidad Católica de Chile, Santiago, 7820436, Chile
[3]Department of Physics, Lehigh University, Bethlehem, Pennsylvania, 18015, USA
[4]Departamento de Física, Universidad Técnica Federico Santa María, Casilla 110, Valparaíso, Chile


February 19, 2026

## Contents


**1 The model** **2**

**2 Renormalization group analysis** **3**

**3 Simple Weyl semimetal** **4**
3.1 Fixing regularization: Coulomb interaction in the instantaneous $(1+1)-$dimensional QED . . . . . 4
3.2 Bosonic self-energy . . . . . 5
3.3 Fermionic self-energy . . . . . 5
3.4 Vertex correction . . . . . 6
3.5 RG equations . . . . . 7

**4 Double Weyl semimetal** **7**
4.1 Bosonic self-energy . . . . . 7
4.2 Fermionic self-energy . . . . . 11
4.3 Vertex correction . . . . . 12
4.4 RG equations . . . . . 12

**5 Triple Weyl semimetal** **13**
5.1 Bosonic self-energy . . . . . 13
5.2 Fermionic self-energy . . . . . 16
5.3 Vertex correction . . . . . 17
5.4 RG equations . . . . . 17

**6 Quadruple Weyl semimetal** **18**
6.1 Bosonic self-energy . . . . . 18
6.2 Fermionic self-energy . . . . . 20
6.3 Vertex correction . . . . . 22
6.4 RG equations . . . . . 22

**7 General Weyl semimetal** **22**
7.1 Bosonic self-energy . . . 22
7.2 Fermionic self-energy . . . 25
7.3 Vertex correction . . . 27
7.4 RG equations . . . 27

**8 Real-space form of the dressed Coulomb interaction and anisotropic screening** **28**
8.1 Irrelevance of quadratic anisotropic term in the Coulomb propagator . . . 28
8.2 Nonanalytic longitudinal screening and real-space form of the dressed interaction for $n > 1$ . . . 28

**9 Logarithmic corrections to observables** **29**
9.1 Renormalized fermion Green's function from the Callan–Symanzik equation . . . 29
9.2 Running effective fine structure constant coupling . . . 30
9.3 Density of states with logarithmic corrections . . . 31
9.4 Specific heat and compressibility . . . 32
9.5 Optical conductivity and its logarithmic corrections . . . 32
9.6 Effective anomalous dimension $\eta_{\psi,\mathrm{eff}}(E)$ . . . 33

# 1 The model

The effective single-particle Hamiltonian describing the low-energy physics of a generalized Weyl semimetal (WSM) with two nodal points characterized by the monopole charges $\pm n$ reads

$$H_n(k_x, k_y, k_z) = A_n k_\perp^n \left[\Gamma_1 \cos(n\phi_k) + \Gamma_2 \sin(n\phi_k)\right] + \Gamma_3 v_z k_z, \tag{1.1}$$

$$\Gamma_1 = \tau_0 \otimes \sigma_1, \quad \Gamma_2 = \tau_0 \otimes \sigma_2, \quad \Gamma_3 = \tau_3 \otimes \sigma_3, \tag{1.2}$$

$$k_\perp^2 = k_x^2 + k_y^2, \quad \phi_k = \tan^{-1}(k_y/k_x). \tag{1.3}$$

For interactions that preserve the chiral symmetry of the system, we can work in a decoupled representation for each of the two-component spinors, in which case the $\Gamma_i$ can be chosen to be the Pauli matrices $\sigma_i$, $\Gamma_i = \sigma_i$, for $i = 1, 2, 3$, which is the representation employed hereafter. We consider instantaneous, long-range Coulomb interaction between such fermions, which is captured by the imaginary time effective action

$$S = \sum_{a=1}^{N} \int d\tau d^3x \psi_a^\dagger \left[(\partial_\tau + ig\Phi) + H_n\right] \psi_a + \frac{1}{2} \int d\tau d^3x \left(\nabla\Phi\right)^2, \tag{1.4}$$

where $\psi_a$ represents the $a$th copy of the Grassmann field labeling each of the $N$ two-component species, and $\Phi$ is the bosonic field that mediates the Coulomb interaction. Casting the action in momentum space, we have

$$S = \sum_{a=1}^{N} \int d^4k\ \psi_{a,k}^\dagger G_0^{-1}(k) \psi_{a,k} + \frac{1}{2} \int d^4k\ D_0^{-1}(k) \Phi_{-k} \Phi_k + ig_0 \sum_{a=1}^{N} \int d^4k d^4q\ \psi_{a,k+q}^\dagger \Phi_q \psi_{a,k}, \tag{1.5}$$

where $k = (k_0, k_x, k_y, k_z)$, with $k_0$ being the zero-temperature ($T = 0$) Matsubara frequency. For future convenience, let us define the vectors $\boldsymbol{k} \equiv (k_0, k_z)$, $\boldsymbol{K} \equiv (k_x, k_y)$, $\boldsymbol{\sigma}_\perp = (\sigma_1, \sigma_2)$ and $\hat{\boldsymbol{n}}_{\boldsymbol{k}} = (\cos(n\phi_k), \sin(n\phi_k))$. The inverse bare fermionic and bosonic propagators are respectively

$$G_0^{-1}(k) = ik_0 + H_n(k_x, k_y, k_z) = ik_0 + \alpha_n |\boldsymbol{K}|^n \boldsymbol{\sigma}_\perp \cdot \hat{\boldsymbol{n}}_{\boldsymbol{k}} + \Gamma_3 v_z k_z, \tag{1.6}$$

$$D_0^{-1}(k) = k_x^2 + k_y^2 + c k_z^2, \tag{1.7}$$

where $c$ is a parameter with bare value $c_0 = 1$ that captures the anisotropy in the bosonic dynamics generated by the fermions with the anisotropic dispersion.

## 2 Renormalization group analysis

In this section we analyze the effects of the Coulomb interaction in a general WSM by employing a renormalization group (RG) procedure controlled by a large $N$ expansion. We implement a controlled large-$N$ expansion with $g^2 \sim 1/N$ and keep the fine structure constant $\alpha_{_N} \equiv Ng^2/v_z$ fixed, so that the polarization bubble is $\mathcal{O}(N^0)$ and is resummed in random phase approximation (RPA), while the fermion self-energy is $\mathcal{O}(1/N)$. In the spirit of a Wilsonian RG scheme, we eliminate the high-energy modes belonging to the shell $\Lambda < E < \Lambda e^{-\ell}$, which transforms the action in Eq. (1.5) into an effective form

$$
\begin{aligned}
S_{\text{eff}} = &\sum_{a=1}^{N} \int d^4k\ \psi^\dagger_{a,k} \left[ik_0(1+\Sigma_0(\ell)) + A_n|\boldsymbol{K}|^n \boldsymbol{\Gamma}\cdot\hat{\boldsymbol{n}}_{\boldsymbol{k}}(1+\Sigma_{12}(\ell)) + \Gamma_3 v_z k_z(1+\Sigma_3(\ell))\right]\psi_{a,k} \\
&+ \frac{1}{2}\int d^4q\ \left[|\boldsymbol{Q}|^2(1+\Pi_{12}(\ell)) + cq_z^2(1+\Pi_3(\ell))\right]\Phi_{-q}\Phi_q + g(1+\delta g(\ell))\sum_{a=1}^{N}\int d^4k d^4q\ \psi^\dagger_{a,k+q}\Phi_q\psi_{a,k},
\end{aligned}
\tag{2.1}
$$

where $\Sigma_0, \Sigma_{12}, \Sigma_3, \Pi_{12}, \Pi_3$ and $\delta g$ are the loop corrections depending on the energy (length) scale controlled by the RG parameter $\ell$. The functional form of the propagators is kept invariant by rescaling the fields as $\psi \to \sqrt{Z_\psi}\psi$ and $\Phi \to \sqrt{Z_\Phi}\Phi$, with $Z_\psi^{-1} = 1+\Sigma_0(\ell)$ and $Z_\Phi^{-1} = 1+\Pi_{12}(\ell)$. The action now reads

$$
\begin{aligned}
S_{\text{eff}} = &\sum_{a=1}^{N} \int d^4k\ \psi^\dagger_{a,k} \left[ik_0 + A_n|\boldsymbol{K}|^n \boldsymbol{\Gamma}\cdot\hat{\boldsymbol{n}}_{\boldsymbol{k}}(1+\Sigma_{12}(\ell)-\Sigma_0(\ell)) + \Gamma_3 v_z k_z(1+\Sigma_3(\ell)-\Sigma_0(\ell))\right]\psi_{a,k} \\
&+ \frac{1}{2}\int d^4q\ \left[|\boldsymbol{Q}|^2 + cq_z^2(1+\Pi_3(\ell)-\Pi_{12}(\ell))\right]\Phi_{-q}\Phi_q \\
&+ g\left(1+\delta g(\ell) - \Sigma_0(\ell) - \frac{\Pi_{12}(\ell)}{2}\right)\sum_{a=1}^{N}\int d^4k d^4q\ \psi^\dagger_{a,k+q}\Phi_q\psi_{a,k}.
\end{aligned}
\tag{2.2}
$$

Assuming that the one-loop corrections have the general form

$$
\Sigma_0(\ell) = \delta g(\ell) = \gamma_0(\ell)\ell, \quad \Sigma_{12}(\ell) = \gamma_{12}(\ell)\ell, \quad \Sigma_3(\ell) = \gamma_3(\ell)\ell, \quad \Pi_{12}(\ell) = \delta_{12}(\ell)\ell, \quad \Pi_3(\ell) = \delta_3(\ell)\ell, \tag{2.3}
$$

where the first equality follows from the Ward-Takahashi identity, the renormalized parameters satisfy the RG equations

$$
\dot{Z}_\psi(\ell) = -\gamma_0(\ell)Z_\psi(\ell), \quad \text{with } Z_\psi(0) = 1, \tag{2.4}
$$

$$
\dot{Z}_\Phi(\ell) = -\delta_{12}(\ell)Z_\Phi(\ell), \quad \text{with } Z_\Phi(0) = 1, \tag{2.5}
$$

$$
\dot{c}(\ell) = \left[\frac{2}{n} - 2 + \delta_3(\ell) - \delta_{12}(\ell)\right]c(\ell), \quad \text{with } c(0) = 1, \tag{2.6}
$$

$$
\dot{A_n}(\ell) = \left[\gamma_{12}(\ell) - \gamma_0(\ell)\right]A_n(\ell), \quad \text{with } A_n(0) = A_n, \tag{2.7}
$$

$$
\dot{v_z}(\ell) = \left[\gamma_3(\ell) - \gamma_0(\ell)\right]v_z(\ell), \quad \text{with } v_z(0) = v_z, \tag{2.8}
$$

$$
\dot{g}(\ell) = -\frac{\delta_{12}(\ell)}{2}g(\ell), \quad \text{with } g(0) = g, \tag{2.9}
$$

as a consequence, we find the $\beta-$function of the effective fine structure constant $\alpha_N = Ng^2/v_z$,

$$
\dot{\alpha}_N(\ell) = -(\delta_{12} - \gamma_3 + \gamma_0)\alpha_N(\ell), \quad \text{with } \alpha_N(0) = \alpha_N^{(0)}. \tag{2.10}
$$

On the other hand, the quadratic piece of the Coulomb propagator $\sim ck_z^2$ is irrelevant at tree level for $n > 1$, as shown in Sec. 8.1, and can therefore be omitted.

# 3 Simple Weyl semimetal

The form of the counterterms, given by Eq. (2.3), in the case of a general WSM in three spatial dimensions depends on the regularization prescription, as it can be explicitly shown. To fix this ambiguity, we require that the regularization is consistent with the U(1) gauge symmetry, i.e., it yields the Ward-Takahashi identity for the instantaneous Coulomb interaction. Since for a general WSM, there is a Lorentz invariant (1+1)-dimensional sector in the plane formed by the imaginary time and $z$ spatial direction, to fix this ambiguity we first consider the version of the $(1+1)-$dimensional Quantum Electrodynamics (QED) with instantaneous electromagnetic interaction.

## 3.1 Fixing regularization: Coulomb interaction in the instantaneous $(1+1)-$dimensional QED

Our regularization scheme relies upon the fact that the loop integrations yield a finite gauge invariant result for the polarization, $\Pi(q)$, in $(1+1)-$dimensional QED [1]. Thus, we first verify that this result holds for the instantaneous interaction in Eq. (1.4) reduced to one spatial dimension:

$$S_0 = \sum_{a=1}^{N} \int d^2k\ \psi^\dagger_{a,k}[ik_0 + v_z k_z \sigma_3]\psi_{a,k} + \frac{1}{2}\int d^2q\ q_z^2 \Phi_{-q}\Phi_q + g_0 \sum_{a=1}^{N}\int d^2k d^2q\ \psi^\dagger_{a,k+q}\Phi_q \psi_{a,k}, \tag{3.1}$$

We compute the density-density correlator, $\Pi(q) \equiv \Pi_{00}(q)$, where $\Pi_{\mu\nu}(q)$ is the polarization tensor, with $\mu, \nu = 0, 1$, in the following three prescriptions:

**(i)** Integrating simultaneously over $k_0$ and $k_z$ yields

$$\begin{aligned}
\Pi(q) &= g^2 \int \mathrm{d}k\, \mathrm{Tr}\big[G_0(k+q)G_0(k)\big] \\
&= 2g^2 \int \frac{d^2k}{(2\pi)^2} \frac{-k_0(k_0+q_0) + v_z^2 k_z(k_z+q_z)}{[(k_0+q_0)^2 + v_z^2(k_z+q_z)^2]\,[k_0^2 + v_z^2 k_z^2]} \\
&= \frac{2g^2}{v_z}\int \frac{d^2k'}{(2\pi)^2}\int_0^1 dx \frac{-k_0'^2 + k_z'^2 + x(1-x)(q_0^2 - v_z^2 q_z^2)}{[k_0'^2 + k_z'^2 + x(1-x)(q_0^2 + v_z^2 q_z^2)]^2} \\
&= \frac{g^2}{2\pi v}\frac{(q_0^2 - v_z^2 q_z^2)}{(q_0^2 + v_z^2 q_z^2)}.
\end{aligned} \tag{3.2}$$

**(ii)** Integrating first over $k_0$ and then over $k_z$ yields

$$\begin{aligned}
\Pi(q) &= \frac{2g^2}{v_z}\int \frac{d^2k'}{(2\pi)^2}\int_0^1 dx \frac{-k_0'^2 + k_z'^2 + x(1-x)(q_0^2 - v_z^2 q_z^2)}{[k_0'^2 + k_z'^2 + x(1-x)(q_0^2 + v_z^2 q_z^2)]^2} \\
&= \frac{g^2}{2v_z}\int_{-\infty}^{\infty}\frac{dk_z'}{2\pi}\int_0^1 dx \frac{-2x(1-x)v_z^2 q_z^2}{[k_z'^2 + x(1-x)(q_0^2 + v_z^2 q_z^2)]^{3/2}} \\
&= \frac{g^2}{\pi v_z}\frac{-v_z^2 q_z^2}{(q_0^2 + v_z^2 q_z^2)}
\end{aligned} \tag{3.3}$$

**(iii)** Integrating first over $k_z$ and then over $k_0$ yields

$$\Pi(q) = \frac{g^2}{\pi v_z}\frac{q_0^2}{(q_0^2 + v_z^2 q_z^2)}. \tag{3.4}$$

We can summarize the result as

$$\Pi(q) = \frac{g^2}{2\pi v_z}\frac{(q_0^2 - v_z^2 q_z^2) + \zeta(q_0^2 + v_z^2 q_z^2)}{(q_0^2 + v_z^2 q_z^2)}, \tag{3.5}$$

where

$$\zeta = \begin{cases} 0, & \text{when integrating over } k_0 \text{ and } k_z \text{ simultaneously} \\ -1, & \text{when integrating first over } k_0 \text{ and then over } k_z \\ +1, & \text{when integrating first over } k_z \text{ and then over } k_0 \end{cases} . \tag{3.6}$$

We note that the prescription of integrating first over $k_0$ ($\zeta = -1$) ensures that the polarization component (3.5) is consistent with the transversality condition, $q^\mu \Pi_{\mu\nu}(q) = 0$, or equivalently, $\Pi_{\mu\nu}(q) = \tilde{\Pi}(q)(\delta_{\mu\nu} - \hat{q}_\mu \hat{q}_\nu)$, in QED when taking $\mu = \nu = 0$. Here, the unit two-vector $\hat{q}_\mu \equiv q_\mu / q$, and $q_\mu = (q_0, v_z q_z)$, with respect to the Euclidean metric $\delta_{\mu\nu}$, implying that $q^2 = \delta_{\mu\nu} q_\mu q_\nu = q_0^2 + v_z^2 q_z^2$.

In the following, we therefore employ the regularization, labeled as "cylindrical" in which we first integrate over frequency, $-\infty < k_0 < \infty$, then over $z-$component of the momentum, $-\infty < k_z < \infty$, and only in the last step we integrate over $(k_x, k_y)$ components of the momentum by imposing a UV momentum cutoff ($\Lambda_\perp$) symmetric with respect to the in-plane rotations, $0 < k_\perp < \Lambda_\perp$, with $k_\perp = \sqrt{k_x^2 + k_y^2}$.

### 3.2 Bosonic self-energy

Next, we analyze the case of a simple ($n = 1$) three-dimensional WSM, for which the Hamiltonian (1.1) takes the form

$$H_1 = A_1 [k_x \sigma_1 + k_y \sigma_2] + v_z k_z \sigma_3, \tag{3.7}$$

and energy dispersion is $E_k = \sqrt{A_1^2 k_x^2 + A_1^2 k_y^2 + v_z^2 k_z^2}$. We compute now compute the polarization (density-density correlator) $\Pi(q)$ using the cylindrical regularization, thus integrating first over $k_0$ and $k_z$ and then imposing an in-plane momentum cutoff $\Lambda_\perp$

$$\begin{aligned}
\Pi(q) &= g^2 \int \mathrm{d}k \, \mathrm{Tr}\big[G_0(k+q) G_0(k)\big] \\
&= 2g^2 N \int \frac{d^4 k}{(2\pi)^4} \frac{-k_0(k_0+q_0) + A_1^2 k_x (k_x+q_x) + A_1^2 k_y (k_y+q_y) + v_z^2 k_z (k_z+q_z)}{[(k_0+q_0)^2 + A_1^2 (k_x+q_x)^2 + A_1^2 (k_y+q_y)^2 + v_z^2 (k_z+q_z)^2]\,\big[k_0^2 + A_1^2 k_x^2 + A_1^2 k_y^2 + v_z^2 k_z^2\big]} \\
&= N \frac{2g^2}{v_z A_1^2} \int \frac{d^4 k'}{(2\pi)^4} \int_0^1 dx \frac{-k_0'^2 + k_z'^2 + k_x'^2 + k_y'^2 + x(1-x)(q_0^2 - E_q^2)}{\big[k_0'^2 + k_z'^2 + k_x'^2 + k_y'^2 + x(1-x)(q_0^2 + E_q^2)\big]^2} \\
&= N \frac{2g^2}{v_z A_1^2} \frac{1}{4\pi} \int \frac{d^2 k'_\perp}{(2\pi)^2} \int_0^1 dx \left\{ \frac{k_x'^2 + k_y'^2 + x(1-x)(q_0^2 - E_q^2)}{k_x'^2 + k_y'^2 + x(1-x)(q_0^2 + E_q^2)} - 1 \right\} \\
&= N \frac{g^2}{4\pi^2 v_z A_1^2} \left[ -\frac{1}{6} E_q^2 \ln\left( \frac{A_1^2 \Lambda_\perp^2}{q_0^2 + E_q^2} \right) - \frac{5}{18} E_q^2 + \mathcal{O}(\Lambda_\perp^{-2}) \right],
\end{aligned} \tag{3.8}$$

which agrees with the results of Ref. [2] up to the numerical coefficient of $E_q^2$ in the finite term when $A_1 = v_z = v$.

The coefficient of the logarithmic divergence in Eq. (3.8) then yields

$$\delta_{12} = \frac{\alpha_N}{12\pi^2}, \quad \delta_3 = \frac{1}{r} \frac{\alpha_N}{12\pi^2} \tag{3.9}$$

where the fine structure constant is defined as $\alpha_N = N g^2 / v_z$, and $r = A_1^2 / v_z^2$ measures the anisotropy of the fermionic dispersion.

### 3.3 Fermionic self-energy

In this section, we compute the one-loop contribution to the fermionic self-energy using the dressed bosonic propagator $D^{-1}(q) = D_0^{-1}(q) - N\Pi(q)$. In Sec. 3.2 we computed polarization $\Pi(q)$ which yields the dressed bosonic propagator

$$D^{-1}(q) = q_x^2 + q_y^2 + c q_z^2 + \alpha_N \frac{\beta}{A_1^2} E_q^2, \tag{3.10}$$

with $\beta = 5/(72\pi^2)$, as given by Eq. (3.8). We now compute the fermionic self-energy $\Sigma(k)$ with the one-loop contribution is given by

$$\begin{aligned}
\Sigma(k) &= (ig)^2 \int \mathrm{d}q\ G_0(k+q)D(q) \\
&= -g^2 \int \mathrm{d}q \frac{-i(k_0+q_0) + A_1(kx+qx)\sigma_1 + A_1(ky+qy)\sigma_2 + v_z(k_z+q_z)\sigma_3}{(k_0+q_0)^2 + A_1^2(k_x+q_x)^2 + A_1^2(k_y+q_y)^2 + v_z^2(k_z+q_z)^2} D(q) \\
&\equiv -\Sigma_0 \cdot ik_0 - \Sigma_1 \cdot A_1 k_x \sigma_1 - \Sigma_2 \cdot A_1 k_y \sigma_2 - \Sigma_3 \cdot v_z k_z \sigma_3
\end{aligned} \tag{3.11}$$

To perform the integrals within the cylindrical regularization, we introduce cylindrical variables, $A_1 q_x = \rho \cos\theta$, $A_1 q_y = \rho \sin\theta$, $v_z q_z = \eta\rho$ and $q_0 = \nu\rho$, such that $E_q^2 = \rho^2(1+\eta^2)$ and in the large $\alpha_N$ limit (keeping $\alpha_N$ fixed)

$$D^{-1}(\rho,\theta,\eta,\nu) = \alpha_N \beta \frac{\rho^2}{A_1^2}(1+\eta^2) \tag{3.12}$$

Setting $k_x = k_y = k_z = 0$ and expanding $G_0(k+q)$ to linear order in $k_0$ yields

$$\Sigma_0 = g^2 \int \mathrm{d}q \frac{q_0^2 - E_q^2}{\left(q_0^2 + E_q^2\right)^2} D(q) = 0 \tag{3.13}$$

Then, setting $k_0 = k_y = k_z = 0$ and expanding $G_0(k+q)$ to linear order in $k_x$ yields

$$\begin{aligned}
\Sigma_1 &= g^2 \int \mathrm{d}q \frac{q_0^2 + v_z^2 q_z^2 + A_1^2 q_y^2 - A_1^2 q_x^2}{\left(q_0^2 + E_q^2\right)^2} D(q) \\
&= \frac{1}{16\pi^4}\frac{1}{\beta N}\int_\omega^{A_1\Lambda_\perp} \frac{d\rho}{\rho}\int_0^{2\pi} d\theta \int_{-\infty}^{\infty} d\eta \int_{-\infty}^{\infty} d\nu\ \frac{\nu^2 + \eta^2 + \left(\sin^2\theta - \cos^2\theta\right)}{\left(\nu^2+\eta^2+1\right)^2}\frac{1}{(1+\eta^2)} \\
&= \frac{1}{6\pi^2\beta}\frac{\ell}{N} = \frac{12}{5}\frac{\ell}{N},
\end{aligned} \tag{3.14}$$

where the RG parameter $\ell \equiv \ln(\Lambda/\omega)$, with $\Lambda = A_1\Lambda_\perp$. By rotational symmetry $\Sigma_2 = \Sigma_1$. Then, setting $k_0 = k_x = k_y = 0$ and expanding $G_0(k+q)$ to linear order in $k_z$ yields

$$\begin{aligned}
\Sigma_3 &= g^2 \int \mathrm{d}q \frac{q_0^2 - v_z^2 q_z^2 + A_1^2 q_y^2 + A_1^2 q_x^2}{\left(q_0^2 + E_q^2\right)^2} D(q) \\
&= \frac{1}{16\pi^4}\frac{1}{\beta N}\int_\omega^{\Lambda} d\rho \int_0^{2\pi} d\theta \int_{-\infty}^{\infty} d\eta \int_{-\infty}^{\infty} d\nu\ \frac{\nu^2 - \eta^2 + 1}{\left(\nu^2+\eta^2+1\right)^2}\frac{1}{(1+\eta^2)} \\
&= \frac{1}{6\pi^2\beta}\frac{\ell}{N} = \frac{12}{5}\frac{\ell}{N}.
\end{aligned} \tag{3.15}$$

Therefore

$$\gamma_0 = 0, \quad \gamma_{12} = \gamma_3 = \frac{12}{5N}. \tag{3.16}$$

### 3.4 Vertex correction

Finally, we verify that the one-loop correction to the vertex at vanishing external momentum and frequency is consistent with the Ward-Takahashi identity

$$\delta g = (ig)^2 \int \mathrm{d}k\ G_0(k)G_0(k)D(k) = g^2 \int \frac{d^4k}{(2\pi)^4}\frac{k_0^2 - E_k^2}{(k_0^2 + E_k^2)^2} D(k) = \Sigma_0 = 0. \tag{3.17}$$

### 3.5 RG equations

Using the RG equations in Eqs. (2.4)-(2.7), and the form of the counterterms found in this section, we obtain

$$\dot{Z}_\psi(\ell) = 0, \tag{3.18}$$

$$\dot{Z}_\Phi(\ell) = -\frac{\alpha_N}{12\pi^2} Z_\Phi(\ell), \tag{3.19}$$

$$\dot{c}(\ell) = -\frac{\alpha_N(\ell)}{12\pi^2}\left(1 - \frac{v^2(\ell)}{A_1^2(\ell)}\right) c(\ell), \tag{3.20}$$

$$\dot{A}_1(\ell) = \frac{12}{5N} A_1(\ell), \tag{3.21}$$

$$\dot{v_z}(\ell) = \frac{12}{5N} v_z(\ell), \tag{3.22}$$

$$\text{and } \dot{\alpha}_N = -\Big(\frac{1}{12\pi^2} + \frac{12}{5N}\Big)\alpha_N^2(\ell) \equiv -F_{\alpha_N}\alpha_N^2(\ell). \tag{3.23}$$

Solving these equations, with bare velocities corresponding to an isotropic simple WSM, $A_1(\ell = 0) = v_z(\ell = 0) \equiv v_0$, we find

$$Z_\psi(\ell) = 1, \tag{3.24}$$

$$Z_\Phi(\ell) = \frac{1}{1 + \frac{1}{12\pi^2}\alpha_N^{(0)}\ell} + \mathcal{O}(1/N), \tag{3.25}$$

$$c(\ell) = 1, \tag{3.26}$$

$$A_1(\ell) = v_z(\ell) = v_0 e^{\gamma_{12}\ell}, \tag{3.27}$$

$$\text{and } \alpha_N(\ell) = \frac{\alpha_N^{(0)}}{1 + \alpha_N^{(0)} F_{\alpha_N}\ell}. \tag{3.28}$$

Notice that the unbounded RG growth of the Fermi velocity in Eq. (3.27) is ultimately cut off once retardation restores the full photon propagator, driving the system to a common terminal velocity shared by the Dirac fermions and photons in the deep infrared [3].

## 4 Double Weyl semimetal

We now focus on the double WSM, for which the Hamiltonian (1.1) reads

$$H_2 = A_2 k_\perp^2 [\sigma_1\cos(2\phi_k) + \sigma_2\sin(2\phi_k)] + v_z k_z \sigma_3, \tag{4.1}$$

where $A_2$ and $v_z$ bear the dimensions of inverse mass and velocity, respectively, and $E_k = \sqrt{A_2^2|\boldsymbol{K}|^4 + v_z^2 k_z^2}$.

### 4.1 Bosonic self-energy

The polarization bubble contribution for each fermionic species is given by

$$\begin{aligned}\Pi(q) &= g^2 \int \mathrm{d}k\, \mathrm{Tr}\big[G_0(k+q)G_0(k)\big] \\ &= 2g^2 \int \frac{d^4k}{(2\pi)^4} \frac{-k_0(k_0+q_0) + A_2^2\boldsymbol{K}^2|\boldsymbol{K}+\boldsymbol{Q}|^2\cos[2(\phi_{k+q}-\phi_k)] + v_z^2 k_z(k_z+q_z)}{[(k_0+q_0)^2 + A_2^2|\boldsymbol{K}+\boldsymbol{Q}|^4 + v_z^2(k_z+q_z)^2]\,[k_0^2 + A_2^2|\boldsymbol{K}|^4 + v_z^2k_z^2]},\end{aligned} \tag{4.2}$$

with the trace computed with one fermion flavor, $N = 1$. We next make use of Feynman parametrization

$$\frac{1}{ab} = \int_0^1 dx \frac{1}{[xa + (1-x)b]^2} \tag{4.3}$$

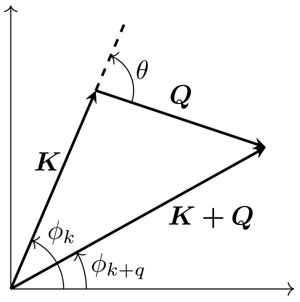


Figure 1: Relevant vectors and angles involved in the calculation of $\Pi(q)$.

and define the scaled momenta $\tilde{\boldsymbol{K}} = \sqrt{A_2}\boldsymbol{K}$, $\tilde{k}_z = v_z k_z$, $\tilde{k}_0 = k_0$. This yields

$$\Pi(\tilde{q}) = \frac{2g^2}{v_z A_2}\int \frac{d^4k'}{(2\pi)^4}\int_0^1 dx \frac{-k_0'^2 + k_z'^2 + \boldsymbol{K}^2|\boldsymbol{K}+\boldsymbol{Q}|^2\cos[2(\phi_{k+q}-\phi_k)] + x(1-x)(q_0^2 - q_z^2)}{\left[k_0'^2 + k_z'^2 + \Delta\left(x,\boldsymbol{K},q\right)\right]^2}, \tag{4.4}$$

where $k_0' = k_0 + xq_0$, $k_z' = k_z + xq_z$ and $\Delta = x(1-x)(q_0^2+q_z^2) + x|\boldsymbol{K}+\boldsymbol{Q}|^4 + (1-x)|\boldsymbol{K}|^4$. Following the prescription justified in Sec. 3, we first integrate analytically over the linear directions $k_0$ and $k_z$ to obtain

$$\Pi(\tilde{q}) = \frac{g^2}{2\pi v_z A_2}\int \frac{d^2\boldsymbol{K}}{(2\pi)^2}\int_0^1 dx \left\{\frac{\boldsymbol{K}^2|\boldsymbol{K}+\boldsymbol{Q}|^2\cos[2(\phi_{k+q}-\phi_k)] + x(1-x)(q_0^2-q_z^2)}{x(1-x)\boldsymbol{q}^2 + x|\boldsymbol{K}+\boldsymbol{Q}|^4 + (1-x)|\boldsymbol{K}|^4} - 1\right\}. \tag{4.5}$$

To proceed with the calculation, we impose a hard UV cutoff $\Lambda_\perp$ in the $\boldsymbol{K}$-space and define dimensionless variables $r = \boldsymbol{K}^2/|\boldsymbol{q}|$, $s = \boldsymbol{Q}^2/|\boldsymbol{q}|$ and $\varphi = \tan^{-1}(q_z/q_0)$. If $\theta$ is the angle between $\boldsymbol{K}$ and $\boldsymbol{Q}$, see Fig. 1, the second term in the numerator can be rewritten as

$$\begin{aligned}
|\boldsymbol{K}|^2|\boldsymbol{K}+\boldsymbol{Q}|^2\cos[2(\phi_{k+q}-\phi_k)] &= 2\left(|\boldsymbol{K}||\boldsymbol{K}+\boldsymbol{Q}|\cos[(\phi_{k+q}-\phi_k)]\right)^2 - |\boldsymbol{K}|^2|\boldsymbol{K}+\boldsymbol{Q}|^2 \\
&= 2\left(\boldsymbol{K}\cdot(\boldsymbol{K}+\boldsymbol{Q})\right)^2 - |\boldsymbol{K}|^2|\boldsymbol{K}+\boldsymbol{Q}|^2 \\
&= \boldsymbol{q}^2\left[r^2 + 2r^{3/2}s^{1/2}\cos\theta + rs\cos 2\theta\right],
\end{aligned} \tag{4.6}$$

while the integration measure reads

$$\int_{|\boldsymbol{K}|<\Lambda_\perp} \frac{d^2\boldsymbol{K}}{(2\pi)^2} \to \frac{|\boldsymbol{q}|}{2(2\pi)}\int_0^{2\pi}\frac{d\theta}{2\pi}\int_0^{\Lambda_r} dr, \tag{4.7}$$

where $\Lambda_r = \Lambda_\perp^2/|\boldsymbol{q}|$. These changes yield

$$\Pi(\tilde{q}) = \frac{g^2}{8\pi^2 v_z A_2}|\boldsymbol{q}|\int_0^{2\pi}\frac{d\theta}{2\pi}\int_0^{\Lambda_r} dr \underbrace{\int_0^1 dx\left\{\frac{r^2 + 2r^{3/2}s^{1/2}\cos\theta + rs\cos 2\theta + x(1-x)\cos 2\varphi}{x(1-x) + x(r + 2r^{1/2}s^{1/2}\cos\theta + s)^2 + (1-x)r^2} - 1\right\}}_{h(r,\theta,s,\varphi)}. \tag{4.8}$$

After integrating over the Feynman parameter we find that $h(r,\theta,s,\varphi)$ has the following asymptotic behavior:

$$h(r,\theta,s,\varphi) = \begin{cases} \mathcal{O}\left(r^0\right), & \text{for } r \ll 1 \\ -\frac{s}{3r}\left(15 - 22|\cos\theta|^2\right) + \mathcal{O}\left(r^{-2}\right), & \text{for } r \gg 1 \end{cases}, \tag{4.9}$$

where we have neglected terms that vanish upon angular integration. To extract the divergent pieces, we define a new function

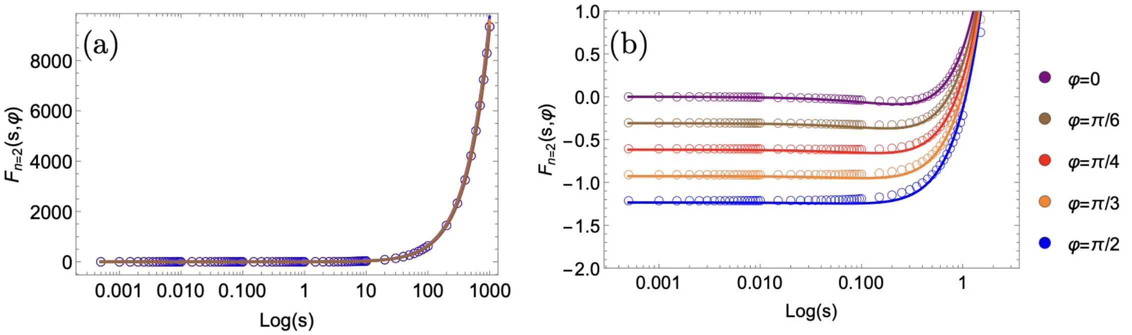


Figure 2: Numerically integrated $F(\Lambda_\perp, s, \varphi)$ (markers) compared to the ansatz $F_{n=2}(\infty, s, \varphi)$ (solid lines) given in Eq. (4.12) for different values of $\varphi$, over (a) a wide range $s \in (10^{-3}, 10^3)$ and (b) small values of $s$.

$$f(r, \theta, s, \varphi) = h(r, \theta, s, \varphi) + \frac{4s}{3\sqrt{r^2+1}}, \tag{4.10}$$

such that $f(r, \theta, s, \varphi)$ gives a finite result when integrated. Our final expression for $\Pi(\tilde{q})$ reads

$$\begin{aligned} \Pi(\tilde{q}) &= \frac{g^2}{8\pi^2 v_z A_2} |\boldsymbol{q}| \int_0^{2\pi} \frac{d\theta}{2\pi} \int_0^{\Lambda_r} dr \left\{ -\frac{4s}{3\sqrt{r^2+1}} + f(r, \theta, s, \varphi) \right\} \\ &= \frac{g^2}{8\pi^2 v_z A_2} \left[ -\frac{4}{3} \boldsymbol{Q}^2 \sinh^{-1}\left( \frac{\Lambda_\perp^2}{|\boldsymbol{q}|} \right) + |\boldsymbol{q}| F(\Lambda_\perp, s, \varphi) \right], \end{aligned} \tag{4.11}$$

where $F(\Lambda_\perp, s, \varphi) = \int_{-\pi}^{\pi} \frac{d\theta}{2\pi} \int_0^{\Lambda_r} dr f(r, \theta, s, \varphi)$ is UV finite, so we only consider the $\mathcal{O}(\Lambda^0)$ contribution given by $F_{n=2}(\infty, s, \varphi) \equiv \lim_{\Lambda_\perp \to \infty} F(\Lambda_\perp, s, \varphi)$. Since this integral is analytically intractable, we propose the ansatz

$$F_{n=2}(\infty, s, \varphi) = -\frac{\pi^2}{8} \sin^2\varphi + \frac{4}{3} s \left[ \ln\left( s + \frac{\pi}{6} \right) + \frac{2}{5} \sin^2\varphi \right], \tag{4.12}$$

which is verified numerically as shown in Fig. 2. We then conclude, using the relation $\sinh^{-1}(z) \approx \ln(2z)$ for $z \gg 1$

$$\Pi(\tilde{q}) = \frac{g^2}{8\pi^2 v_z A_2} \left[ -\frac{\pi^2}{8} \frac{q_z^2}{|\boldsymbol{q}|} - \frac{4}{3} \boldsymbol{Q}^2 \ln\left( \frac{\Lambda_\perp^2}{|\boldsymbol{q}|} \right) + \frac{4}{3} \boldsymbol{Q}^2 \ln\left( \frac{\boldsymbol{Q}^2}{|\boldsymbol{q}|} + \frac{\pi}{6} \right) + \frac{4}{3} \boldsymbol{Q}^2 \left( \frac{2}{5} \sin^2\varphi - \ln 2 \right) \right]. \tag{4.13}$$

In terms of the unscaled momenta, we find

$$\begin{aligned} \Pi(q) &= -\frac{g^2}{64 v_z A_2} \frac{v_z^2 q_z^2}{\sqrt{q_0^2 + v_z^2 q_z^2}} - \frac{g^2}{6\pi^2 v_z} \boldsymbol{Q}^2 \left[ \ln\left( \frac{A_2 \Lambda_\perp^2}{A_2 \boldsymbol{Q}^2 + (\pi/6)\sqrt{q_0^2 + v_z^2 q_z^2}} \right) - \left( \frac{2}{5} \frac{v_z^2 q_z^2}{q_0^2 + v_z^2 q_z^2} - \ln 2 \right) \right], \end{aligned} \tag{4.14}$$

$$= -\frac{g^2}{64 v_z A_2} \frac{v_z^2 q_z^2}{\sqrt{q_0^2 + v_z^2 q_z^2}} - \frac{g^2}{6\pi^2 v_z} \boldsymbol{Q}^2 \left[ \ln\left( \frac{\Lambda}{A_2 \boldsymbol{Q}^2 + (\pi/6)\sqrt{q_0^2 + v_z^2 q_z^2}} \right) - \left( \frac{2}{5} \frac{v_z^2 q_z^2}{q_0^2 + v_z^2 q_z^2} - \ln 2 \right) \right], \tag{4.15}$$

where $\Lambda$ is the energy cutoff, yielding the form of the counterterms

$$\delta_{12} = \frac{\alpha_N}{6\pi^2}, \text{and} \qquad \delta_3 = 0. \tag{4.16}$$

Next, we verify that the result given in Eq. (4.14) satisfies the limiting cases (i) $q = 0$, (ii) $\boldsymbol{q} = 0$ and (iii) $\boldsymbol{Q} = 0$.

**(i)** $q = 0$**:**

$$\Pi(\tilde{q} = 0) = 0 \tag{4.17}$$

**(ii) $\boldsymbol{q} = 0$:**

$$\begin{aligned}
\Pi(\tilde{\boldsymbol{q}}=0,\tilde{\boldsymbol{Q}}) &= \frac{g^2}{2\pi v_z A_2}\int\frac{d^2\boldsymbol{K}}{(2\pi)^2}\int_0^1 dx\left\{\frac{\boldsymbol{K}^2|\boldsymbol{K}+\boldsymbol{Q}|^2\cos[2(\phi_{k+q}-\phi_k)]}{x|\boldsymbol{K}+\boldsymbol{Q}|^4+(1-x)|\boldsymbol{K}|^4}-1\right\}\\
&= \frac{g^2}{2\pi v_z A_2}\int\frac{d^2\boldsymbol{K}}{(2\pi)^2}\left\{\frac{\boldsymbol{K}^2|\boldsymbol{K}+\boldsymbol{Q}|^2\cos[2(\phi_{k+q}-\phi_k)]}{|\boldsymbol{K}+\boldsymbol{Q}|^4-|\boldsymbol{K}|^4}\ln\left(\frac{|\boldsymbol{K}+\boldsymbol{Q}|^4}{|\boldsymbol{K}|^4}\right)-1\right\}\\
&= \frac{g^2}{2\pi v_z A_2}\int\frac{d^2\boldsymbol{K}}{(2\pi)^2}\left\{\frac{2\left(\boldsymbol{K}\cdot(\boldsymbol{K}+\boldsymbol{Q})\right)^2-|\boldsymbol{K}|^2|\boldsymbol{K}+\boldsymbol{Q}|^2}{|\boldsymbol{K}+\boldsymbol{Q}|^4-|\boldsymbol{K}|^4}\ln\left(\frac{|\boldsymbol{K}+\boldsymbol{Q}|^4}{|\boldsymbol{K}|^4}\right)-1\right\},
\end{aligned}$$

with variable shifted $\boldsymbol{K}\to\boldsymbol{K}-\boldsymbol{Q}/2$,

$$\begin{aligned}
&= \frac{g^2}{2\pi v_z A_2}\int\frac{d^2\boldsymbol{K}}{(2\pi)^2}\left\{\frac{2\left(\boldsymbol{K}^2-\boldsymbol{Q}^2/4\right)^2-|\boldsymbol{K}-\boldsymbol{Q}/2|^2|\boldsymbol{K}+\boldsymbol{Q}/2|^2}{|\boldsymbol{K}+\boldsymbol{Q}/2|^4-|\boldsymbol{K}-\boldsymbol{Q}/2|^4}\ln\left(\frac{|\boldsymbol{K}+\boldsymbol{Q}/2|^4}{|\boldsymbol{K}-\boldsymbol{Q}/2|^4}\right)-1\right\}\\
&= \frac{g^2}{2\pi v_z A_2}\int\frac{d^2\boldsymbol{K}}{(2\pi)^2}\int_0^1 dx\left\{\frac{|\boldsymbol{K}|^4+|\boldsymbol{Q}|^4/16-3\boldsymbol{K}^2\boldsymbol{Q}^2/2+(\boldsymbol{K}\cdot\boldsymbol{Q})^2}{2(\boldsymbol{K}\cdot\boldsymbol{Q})(2\boldsymbol{K}^2+\boldsymbol{Q}^2/2)}\frac{4\boldsymbol{Q}\cdot\boldsymbol{K}}{2x\boldsymbol{Q}\cdot\boldsymbol{K}+|\boldsymbol{K}-\boldsymbol{Q}/2|^2}-1\right\}\\
&= \frac{g^2}{2\pi v_z A_2}\int\frac{d^2\boldsymbol{K}}{(2\pi)^2}\int_0^1 dxdy\left\{\frac{|\boldsymbol{K}|^4+|\boldsymbol{Q}|^4/16-3\boldsymbol{K}^2\boldsymbol{Q}^2/2+(\boldsymbol{K}\cdot\boldsymbol{Q})^2}{\left[\boldsymbol{K}^2+y(2x-1)\boldsymbol{K}\cdot\boldsymbol{Q}+\boldsymbol{Q}^2/4\right]^2}-1\right\},
\end{aligned}$$

with a new variable $z=y(2x-1)$,

$$= \frac{g^2}{2\pi v_z A_2}\int\frac{d^2\boldsymbol{K}}{(2\pi)^2}\int_0^1 dxdy\left\{\frac{-2\boldsymbol{K}^2\boldsymbol{Q}^2+(1-z^2)(\boldsymbol{K}\cdot\boldsymbol{Q})^2-2z(\boldsymbol{K}^2+\boldsymbol{Q}^2/4)(\boldsymbol{K}\cdot\boldsymbol{Q})}{\left[\boldsymbol{K}^2+z\boldsymbol{K}\cdot\boldsymbol{Q}+\boldsymbol{Q}^2/4\right]^2}\right\}$$

and after a substitution $\boldsymbol{K'}=\boldsymbol{K}+\frac{z}{2}\boldsymbol{Q}$

$$= \frac{g^2}{2\pi v_z A_2}\int\frac{d^2\boldsymbol{K'}}{(2\pi)^2}\int_0^1 dxdy\quad\left\{\frac{(z^2-2)\boldsymbol{K'}^2\boldsymbol{Q}^2+(1+z^2)(\boldsymbol{K'}\cdot\boldsymbol{Q})^2}{\left[\boldsymbol{K'}^2+(1-z^2)\boldsymbol{Q}^2/4\right]^2}\right\},$$

using that under the intergral , because of rotational symmetry $K'_iK'_j\to\frac{\boldsymbol{K'}^2}{2}\delta_{ij}$,

$$\begin{aligned}
&= \frac{g^2}{2\pi v_z A_2}\int\frac{d^2\boldsymbol{K'}}{(2\pi)^2}\int_0^1 dxdy\quad\left\{\frac{3(z^2-1)/2\boldsymbol{K'}^2\boldsymbol{Q}^2}{\left[\boldsymbol{K'}^2+(1-z^2)\boldsymbol{Q}^2/4\right]^2}\right\}\\
&= \frac{g^2}{2\pi v_z A_2}\boldsymbol{Q}^2\int_0^1 dxdy\frac{3(z^2-1)}{2}\frac{1}{4\pi}\left\{-1+\ln\Lambda_\perp^2-\ln[(1-z^2)\boldsymbol{Q}^2/4]\right\}\\
&= -\frac{g^2}{6\pi^2 v_z A_2}\boldsymbol{Q}^2\left[\ln\frac{\Lambda^2}{\boldsymbol{Q}^2}+\mathcal{O}(1)\right].
\end{aligned}\tag{4.18}$$

**(iii) $\boldsymbol{Q} = 0$:**

$$\begin{aligned}
\Pi(\tilde{\boldsymbol{q}},\tilde{\boldsymbol{Q}}=0) &= \frac{g^2}{2\pi v_z A_2}\int\frac{d^2\boldsymbol{K}}{(2\pi)^2}\int_0^1 dx\left\{\frac{|\boldsymbol{K}|^4+x(1-x)(q_0^2-q_z^2)}{x(1-x)\boldsymbol{q}^2+|\boldsymbol{K}|^4}-1\right\}\\
&= \frac{g^2}{2\pi v_z A_2}\int\frac{d^2\boldsymbol{K}}{(2\pi)^2}\int_0^1 dx\left\{\frac{-2x(1-x)q_z^2}{x(1-x)\boldsymbol{q}^2+|\boldsymbol{K}|^4}\right\}\\
&= \frac{g^2}{8\pi v_z A_2}\frac{q_z^2}{|\boldsymbol{q}|}\int_0^1 dx\left[\sqrt{\frac{x^3}{1-x}}-\sqrt{\frac{x}{1-x}}\right]\\
&= -\frac{g^2}{64 v_z A_2}\frac{q_z^2}{|\boldsymbol{q}|}
\end{aligned}\tag{4.19}$$

## 4.2 Fermionic self-energy

The first order contribution to the fermionic self-energy is

$$\begin{aligned}\Sigma(k) &= (ig)^2 \int \mathrm{d}q\ G_0(k+q)D(q) \\ &= -g^2 \int \mathrm{d}q \frac{-i(k_0+q_0) + A_2|\boldsymbol{K}+\boldsymbol{Q}|^2[\sigma_1\cos(2\phi_{k+q}) + \sigma_2\sin(2\phi_{k+q})] + v_z(k_z+q_z)\sigma_3}{(k_0+q_0)^2 + A_2^2|\boldsymbol{K}+\boldsymbol{Q}|^4 + v_z^2(k_z+q_z)^2} D(q) \\ &\equiv -\Sigma_0\cdot ik_0 - \Sigma_{12}\cdot A_2\boldsymbol{K}^2[\sigma_1\cos(2\phi_k)+\sigma_2\sin(2\phi_k)] - \Sigma_3\cdot v_zk_z\sigma_3 \end{aligned} \tag{4.20}$$

where $D^{-1}(q) = D_0^{-1}(q) - N\Pi(q)$. After absorbing the cutoff-dependent terms in Eq. (4.14) in the counter-terms of the renormalized theory, the dressed bosonic propagator reads

$$D^{-1}(q) = \boldsymbol{Q}^2 + cq_z^2 + \frac{\alpha_N}{64A_2}\frac{v_z^2q_z^2}{\sqrt{q_0^2+v_z^2q_z^2}} - \frac{\alpha_N}{6\pi^2}\boldsymbol{Q}^2\left(\frac{2}{5}\frac{v_z^2q_z^2}{q_0^2+v_z^2q_z^2} - \ln 2\right). \tag{4.21}$$

To be consistent with the regularization employed in Sec. 4.1, we compute $\Sigma(k)$ by integrating first over $k_0$, then over $k_z$ and finally imposing an in-plane cutoff $\omega < A_2\boldsymbol{K}^2 < \Lambda = A_2\Lambda_\perp^2$. Let us define new variables as

$$\begin{cases}\sqrt{A_2}Q_x = \rho^{1/2}\cos\theta, \\ \sqrt{A_2}Q_y = \rho^{1/2}\sin\theta, \\ v_zq_z = \eta\rho, \\ q_0 = \nu\rho. \end{cases} \tag{4.22}$$

We can then rewrite the propagator as $D^{-1}(q) = A_2^{-1}\rho d^{-1}(q)$, where

$$d^{-1}(\rho,\phi,\theta,\nu) = \sin\phi + c\frac{A_2}{v_z^2}\rho\eta^2 + \alpha_N\left[\frac{\eta^2}{64\sqrt{\nu^2+\eta^2}} - \frac{1}{6\pi^2}\left(\frac{2}{5}\frac{\eta^2}{\nu^2+\eta^2} - \ln 2\right)\right]. \tag{4.23}$$

**(i) $\Sigma_0$:**

Here we set $\boldsymbol{K}=0$, $k_z=0$ and expand $G_0(k+q)$ to linear order in $k_0$, which yields

$$\begin{aligned}\Sigma_0 &= g^2\int \mathrm{d}q \frac{q_0^2 - A_2^2\boldsymbol{Q}^4 - v_z^2q_z^2}{\left(q_0^2+A_2^2\boldsymbol{Q}^4+v_z^2q_z^2\right)^2}D(q) \\ &= \frac{1}{N(2\pi)^3}\int_\omega^\Lambda \frac{d\rho}{\rho}\int_{-\infty}^{\infty} d\eta \int_{-\infty}^{\infty} d\nu \frac{1}{2}\frac{\nu^2-\eta^2-1}{\left(\nu^2+\eta^2+1\right)^2}\left[\frac{\eta^2}{64\sqrt{\nu^2+\eta^2}} - \frac{1}{6\pi^2}\left(\frac{2}{5}\frac{\eta^2}{\nu^2+\eta^2} - \ln 2\right)\right]^{-1} + \mathcal{O}(\alpha_N^{-1}) \\ &= 0.344\frac{\ell}{N} \end{aligned} \tag{4.24}$$

**(ii) $\Sigma_3$:**

Here we set $\boldsymbol{K}=0$, $k_0=0$ and expand $G_0(k+q)$ to linear order in $k_z$, which yields

$$\begin{aligned}\Sigma_3 &= g^2\int \mathrm{d}q \frac{q_0^2 + A_2^2\boldsymbol{Q}^4 - v_z^2q_z^2}{\left(q_0^2+A_2^2\boldsymbol{Q}^4+v_z^2q_z^2\right)^2}D(q) \\ &= \frac{1}{N(2\pi)^3}\int_\omega^\Lambda \frac{d\rho}{\rho}\int_{-\infty}^{\infty} d\eta \int_{-\infty}^{\infty} d\nu \frac{1}{2}\frac{\nu^2+1-\eta^2}{\left(\nu^2+\eta^2+1\right)^2}\left[\frac{\eta^2}{64\sqrt{\nu^2+\eta^2}} - \frac{1}{6\pi^2}\left(\frac{2}{5}\frac{\eta^2}{\nu^2+\eta^2} - \ln 2\right)\right]^{-1} + \mathcal{O}(\alpha_N^{-1}) \\ &= 1.172\frac{\ell}{N} \end{aligned} \tag{4.25}$$

**(iii) $\Sigma_{12}$:**

Here it is convenient to rewrite the second term in Eq. (4.20) as

$$\Sigma_{12}\cdot A_2\boldsymbol{K}^2[\sigma_1\cos(2\phi_k)+\sigma_2\sin(2\phi_k)]\equiv\Sigma_1\cdot A_2(K_x^2-K_y^2)\sigma_1+\Sigma_2\cdot A_2 2K_xK_y\sigma_2. \tag{4.26}$$

Since rotational symmetry enforces $\Sigma_1=\Sigma_2=\Sigma_{12}$, we show only the computation of $\Sigma_2$. Setting $k_0=0$, $k_z=0$ and expanding $G_0(k+q)$ to second order in $K_x$ and $K_y$ yields

$$\begin{aligned}\Sigma_2&=g^2\int \mathrm{d}q\,\frac{\left(-3A_2^2(q_x^2+q_y^2)^2+v_z^2q_z^2+q_0^2\right)\left(A_2^2(-6q_x^2q_y^2+q_x^4+q_y^4)+v_z^2q_z^2+q_0^2\right)}{\left(A_2^2(q_x^2+q_y^2)^2+v_z^2q_z^2+q_0^2\right)^3}D(q)\\&=\frac{1}{N(2\pi)^4}\int_\omega^\Lambda\frac{d\rho}{\rho}\int_0^{2\pi}d\theta\int_{-\infty}^{\infty}d\eta\int_{-\infty}^{\infty}d\nu\,\frac{(\eta^2+\nu^2-3)\,(\eta^2+\nu^2+\cos 4\theta)}{\rho^2(\eta^2+\nu^2+1)^3}\\&\quad\times\frac{1}{\frac{\eta^2}{64\sqrt{\nu^2+\eta^2}}-\frac{1}{6\pi^2}\left(\frac{2}{5}\frac{\eta^2}{\nu^2+\eta^2}-\ln 2\right)}\;+\;\mathcal{O}(\alpha_N^{-1})=0.747\,\frac{\ell}{N}.\end{aligned}\tag{4.27}$$

Therefore, we obtain

$$\gamma_0=\frac{0.344}{N},\quad \gamma_{12}=\frac{1.172}{N},\ \text{and}\ \gamma_3=\frac{0.747}{N}. \tag{4.28}$$

## 4.3 Vertex correction

Finally, we verify that the one-loop correction to the vertex at vanishing external momentum and frequency is consistent with the Ward-Takahashi identity

$$\delta g=(ig)^2\int \mathrm{d}k\;G_0(k)G_0(k)D(k)=g^2\int\frac{d^4k}{(2\pi)^4}\frac{k_0^2-E_k^2}{\left(k_0^2+E_k^2\right)^2}D(k)=\Sigma_0=0.344\frac{\ell}{N} \tag{4.29}$$

## 4.4 RG equations

Using the RG equations in Eqs. (2.4)-(2.7), and the form of the counterterms found in this section, we obtain

$$\dot{Z}_\psi(\ell)=-\gamma_0Z_\psi(\ell), \tag{4.30}$$
$$\dot{A}_2(\ell)=(\gamma_{12}-\gamma_0)A_2(\ell), \tag{4.31}$$
$$\dot{v_z}(\ell)=(\gamma_3-\gamma_0)v_z(\ell), \tag{4.32}$$
$$\text{and }\dot{\alpha}_N(\ell)=-\frac{\alpha_N^2(\ell)}{3\pi^2}+\mathcal{O}(1/N), \tag{4.33}$$

with $\gamma_a$ $(a=0,12,3)$ given by Eq. (4.28), and the value of $\delta_a$ $(a=12,3)$ in Eq. (4.16).

Solving these equations we obtain

$$Z_\psi(\ell)=e^{-\gamma_0\ell}, \tag{4.34}$$
$$A_2(\ell)=A_2e^{(\gamma_{12}-\gamma_0)\ell}, \tag{4.35}$$
$$v_z(\ell)=v_ze^{(\gamma_3-\gamma_0)\ell}, \tag{4.36}$$
$$\text{and }\alpha_N(\ell)=\frac{\alpha_N^{(0)}}{1+\frac{\alpha_N^{(0)}}{6\pi^2}\ell}. \tag{4.37}$$

# 5 Triple Weyl semimetal

We now focus on the triple WSM, for which the Hamiltonian (1.1) reads

$$H_3 = A_3 k_\perp^3 [\sigma_1 \cos(3\phi_k) + \sigma_2 \sin(3\phi_k)] + v_z k_z \sigma_3, \tag{5.1}$$

and the energy dispersion is $E_k = \sqrt{A_3^2 |\boldsymbol{K}|^6 + v_z^2 k_z^2}$.

## 5.1 Bosonic self-energy

The polarization bubble contribution for each fermionic species is given by

$$\begin{aligned}
\Pi(q) &= g^2 \int \mathrm{d}k \, \mathrm{Tr}\big[G_0(k+q) G_0(k)\big] \\
&= 2g^2 \int \frac{d^4k}{(2\pi)^4} \frac{-k_0(k_0+q_0) + A_3^2 |\boldsymbol{K}|^3 |\boldsymbol{K}+\boldsymbol{Q}|^3 \cos[3(\phi_{k+q} - \phi_k)] + v_z^2 k_z (k_z + q_z)}{[(k_0+q_0)^2 + A_3^2 |\boldsymbol{K}+\boldsymbol{Q}|^6 + v_z^2 (k_z+q_z)^2]\,[k_0^2 + A_3^2 |\boldsymbol{K}|^6 + v_z^2 k_z^2]}.
\end{aligned} \tag{5.2}$$

We next make use of Feynman parametrization

$$\frac{1}{ab} = \int_0^1 dx \frac{1}{[xa + (1-x)b]^2} \tag{5.3}$$

and define the scaled momenta $\tilde{\boldsymbol{K}} = A_3^{1/3} \boldsymbol{K}$, $\tilde{k_z} = v_z k_z$, $\tilde{k_0} = k_0$. This yields

$$\Pi(\tilde{q}) = \frac{2g^2}{v_z A_3^{2/3}} \int \frac{d^4k'}{(2\pi)^4} \int_0^1 dx \frac{-k_0'^2 + k_z'^2 + |\boldsymbol{K}|^3 |\boldsymbol{K}+\boldsymbol{Q}|^3 \cos[3(\phi_{k+q} - \phi_k)] + x(1-x)(q_0^2 - q_z^2)}{[k_0'^2 + k_z'^2 + \Delta\,(x, \boldsymbol{K}, q)]^2}, \tag{5.4}$$

where $k_0' = k_0 + x q_0$, $k_z' = k_z + x q_z$ and $\Delta = x(1-x)(q_0^2 + q_z^2) + x|\boldsymbol{K}+\boldsymbol{Q}|^6 + (1-x)|\boldsymbol{K}|^6$. Following the prescription justified in Sec. 3, we first integrate analytically over the linear directions $k_0$ and $k_z$ to obtain

$$\Pi(\tilde{q}) = \frac{g^2}{2\pi v_z A_3^{2/3}} \int \frac{d^2\boldsymbol{K}}{(2\pi)^2} \int_0^1 dx \left\{ \frac{|\boldsymbol{K}|^3 |\boldsymbol{K}+\boldsymbol{Q}|^3 \cos[3(\phi_{k+q} - \phi_k)] + x(1-x)(q_0^2 - q_z^2)}{x(1-x)\boldsymbol{q}^2 + x|\boldsymbol{K}+\boldsymbol{Q}|^6 + (1-x)|\boldsymbol{K}|^6} - 1 \right\}. \tag{5.5}$$

To proceed with the calculation, we impose a hard UV cutoff $\Lambda_\perp$ in the $\boldsymbol{K}$-space and define dimensionless variables $r = \boldsymbol{K}^2/|\boldsymbol{q}|^{2/3}$, $s = \boldsymbol{Q}^2/|\boldsymbol{q}|^{2/3}$ and $\varphi = \tan^{-1}(q_z/q_0)$. If $\theta$ is the angle between $\boldsymbol{K}$ and $\boldsymbol{Q}$, see Fig. 1, using the identity $\cos(3x) = 4\cos^3 x - 3\cos x$ the second term in the numerator can be rewritten as

$$\begin{aligned}
|\boldsymbol{K}|^3 |\boldsymbol{K}+\boldsymbol{Q}|^3 \cos\big[3(\phi_{k+q} - \phi_k)\big] &= \Big(|\boldsymbol{K}||\boldsymbol{K}+\boldsymbol{Q}| \cos(\phi_{k+q} - \phi_k)\Big) \\
&\times \left(4\Big(|\boldsymbol{K}||\boldsymbol{K}+\boldsymbol{Q}| \cos(\phi_{k+q} - \phi_k)\Big)^2 - 3|\boldsymbol{K}|^2 |\boldsymbol{K}+\boldsymbol{Q}|^2\right) \\
&= \Big(|\boldsymbol{K}|^2 + |\boldsymbol{K}||\boldsymbol{Q}| \cos\theta\Big)\left(4\Big(|\boldsymbol{K}|^2 + |\boldsymbol{K}||\boldsymbol{Q}| \cos\theta\Big)^2 - 3|\boldsymbol{K}|^2 |\boldsymbol{K}+\boldsymbol{Q}|^2\right) \\
&= |\boldsymbol{q}|^2 \Big(r^3 + 3r^{5/2} s^{1/2} \cos\theta + 3r^2 s \cos(2\theta) + r^{3/2} s^{3/2} \cos(3\theta)\Big).
\end{aligned} \tag{5.6}$$

while the integration measure reads

$$\int_{|\boldsymbol{K}| < \Lambda_\perp} \frac{d^2\boldsymbol{K}}{(2\pi)^2} \to \frac{|\boldsymbol{q}|^{2/3}}{2(2\pi)} \int_0^{2\pi} \frac{d\theta}{2\pi} \int_0^{\Lambda_r} dr, \tag{5.7}$$

where $\Lambda_r = \Lambda_\perp^2/|\boldsymbol{q}|^{2/3}$. These changes yield

$$\Pi(\tilde{q}) = \frac{g^2}{8\pi^2 v_z A_3^{2/3}} |\boldsymbol{q}|^{2/3} \int_0^{2\pi} \frac{d\theta}{2\pi} \int_0^{\Lambda_r} dr \underbrace{\int_0^1 dx \left\{ \mathcal{N}(r,\theta,s,\varphi;x)\, \mathcal{D}(r,\theta,s,\varphi;x)^{-1} - 1 \right\}}_{h(r,\theta,s,\varphi)}, \tag{5.8}$$

where $\mathcal{N} \equiv r^3 + 3r^{5/2}s^{1/2}\cos\theta + 3r^2 s\cos(2\theta) + r^{3/2}s^{3/2}\cos(3\theta) + x(1-x)\cos 2\varphi,$

and $\mathcal{D} \equiv x(1-x) + x\left(r + 2r^{1/2}s^{1/2}\cos\theta + s\right)^3 + (1-x)r^3.$

After integrating over the Feynman parameter we find that $h(r,\theta,s,\varphi)$ has the following asymptotic behavior:

$$h(r,\theta,s,\varphi) = \begin{cases} \mathcal{O}\left(r^0\right), & \text{for } r \ll 1 \\ -\frac{s}{2r}\left(9 - 6|\cos\theta|^2\right) + \mathcal{O}\left(r^{-2}\right), & \text{for } r \gg 1 \end{cases}, \tag{5.9}$$

where we have neglected terms that vanish upon angular integration. To extract the divergent pieces, we define a new function

$$f(r,\theta,s,\varphi) = h(r,\theta,s,\varphi) + \frac{3s}{\sqrt{r^2+1}}, \tag{5.10}$$

such that $f(r,\theta,s,\varphi)$ gives a finite result when integrated. Our final expression for $\Pi(\tilde{q})$ reads

$$\begin{aligned} \Pi(\tilde{q}) &= \frac{g^2}{8\pi^2 v_z A_3^{2/3}} |\boldsymbol{q}|^{2/3} \int_0^{2\pi} \frac{d\theta}{2\pi} \int_0^{\Lambda_r} dr \left\{ -\frac{3s}{\sqrt{r^2+1}} + f(r,\theta,s,\varphi) \right\} \\ &= \frac{g^2}{8\pi^2 v_z A_3^{2/3}} \left[ -3\boldsymbol{Q}^2 \sinh^{-1}\left(\frac{\Lambda_\perp^2}{|\boldsymbol{q}|^{2/3}}\right) + |\boldsymbol{q}|^{2/3} F(\Lambda_\perp, s, \varphi) \right], \end{aligned} \tag{5.11}$$

where $F(\Lambda_\perp, s, \varphi) = \int_{-\pi}^{\pi} \frac{d\theta}{2\pi} \int_0^{\Lambda_r} dr f(r,\theta,s,\varphi)$ is UV finite, so we only consider the $\mathcal{O}(\Lambda_\perp^0)$ contribution given by $F_{n=3}(\infty, s, \varphi) \equiv \lim_{\Lambda_\perp \to \infty} F(\Lambda_\perp, s, \varphi)$. Since this integral is analytically intractable, we propose the ansatz

$$F_{n=3}(\infty, s, \varphi) = -8\pi^2 b_3^{(1)} \sin^2\varphi + 3s\left[\ln\left(s + \frac{5}{4}\right) + \frac{1}{4}\sin^2\varphi\right], \tag{5.12}$$

where

$$b_3^{(1)} = \frac{\Gamma\left(\frac{4}{3}\right)^2}{6\pi\sqrt{3}\,\Gamma\left(\frac{8}{3}\right)} \approx 0.016. \tag{5.13}$$

The ansatz is verified numerically as shown in Fig. 3. We then conclude, using the relation $\sinh^{-1}(z) \approx \ln(2z)$ for $z \gg 1$:

$$\Pi(\tilde{q}) = \frac{g^2}{8\pi^2 v_z A_3^{2/3}} \left[ -8\pi^2 b_3^{(1)} \frac{q_z^2}{|\boldsymbol{q}|^{4/3}} - 3\boldsymbol{Q}^2 \ln\left(\frac{\Lambda_\perp^2}{|\boldsymbol{q}|^{2/3}}\right) + 3\boldsymbol{Q}^2 \ln\left(\frac{\boldsymbol{Q}^2}{|\boldsymbol{q}|^{2/3}} + \frac{5}{4}\right) + 3\boldsymbol{Q}^2\left(\frac{1}{4}\sin^2\varphi - \ln 2\right) \right]. \tag{5.14}$$

In terms of the unscaled momenta:

$$\begin{aligned} \Pi(q) &= -b_3^{(1)} \frac{g^2}{v_z A_3^{2/3}} \frac{v_z^2 q_z^2}{(q_0^2 + v_z^2 q_z^2)^{2/3}} - \frac{3g^2}{8\pi^2 v_z} \boldsymbol{Q}^2 \left[ \ln\left( \frac{A_3^{2/3}\Lambda_\perp^2}{A_3^{2/3}\boldsymbol{Q}^2 + (5/4)(q_0^2 + v_z^2 q_z^2)^{1/3}} \right) - \left(\frac{1}{4}\sin^2\varphi - \ln 2\right) \right] & (5.15) \\ &= -b_3^{(1)} \frac{g^2}{v_z A_3^{2/3}} \frac{v_z^2 q_z^2}{(q_0^2 + v_z^2 q_z^2)^{2/3}} - \frac{3g^2}{8\pi^2 v_z} \boldsymbol{Q}^2 \left[ \ln\left( \frac{\Lambda^{2/3}}{A_3^{2/3}\boldsymbol{Q}^2 + (5/4)(q_0^2 + v_z^2 q_z^2)^{1/3}} \right) - \left(\frac{1}{4}\sin^2\varphi - \ln 2\right) \right] & (5.16) \end{aligned}$$

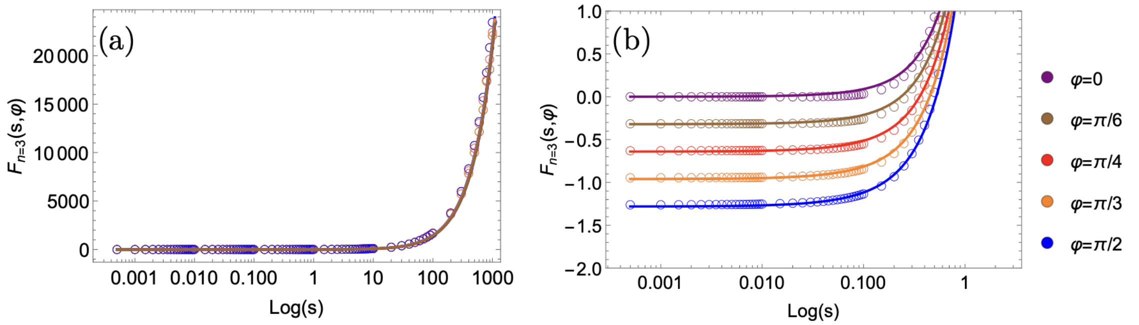


Figure 3: Numerically integrated $F(\Lambda_\perp, s, \varphi)$ (markers) compared to the ansatz $F_{n=3}(\infty, s, \varphi)$ (solid lines) given in Eq. (5.12) for different values of $\varphi$, over (a) a wide range $s \in (10^{-3}, 10^3)$ and (b) small values of $s$.

Therefore, we obtain

$$\delta_{12} = \frac{\alpha_N}{4\pi^2} \text{ and } \delta_3 = 0. \tag{5.17}$$

Next, we verify that the result given in Eq. (5.15) satisfies the limiting cases (i) $q = 0$, (ii) $\boldsymbol{q} = 0$ and (iii) $\boldsymbol{Q} = 0$.

**(i) $q = 0$:**

$$\Pi(\tilde{q} = 0) = 0 \tag{5.18}$$

**(ii) $\boldsymbol{q} = 0$:**

$$\begin{aligned}\Pi(\tilde{\boldsymbol{q}} = 0, \tilde{\boldsymbol{Q}}) &= \frac{g^2}{2\pi v_z A_3^{2/3}} \int \frac{d^2\boldsymbol{K}}{(2\pi)^2} \int_0^1 dx \left\{ \frac{|\boldsymbol{K}|^3 |\boldsymbol{K}+\boldsymbol{Q}|^3 \cos[3(\phi_{k+q} - \phi_k)]}{x|\boldsymbol{K}+\boldsymbol{Q}|^6 + (1-x)|\boldsymbol{K}|^6} - 1 \right\} \\ &= -\frac{3g^2}{8\pi^2 v_z} \boldsymbol{Q}^2 \left[ \ln\left( \frac{\Lambda_\perp^2}{\boldsymbol{Q}^2} \right) + \mathcal{O}(1) \right]\end{aligned} \tag{5.19}$$

**(iii) $\boldsymbol{Q} = 0$:**

$$\begin{aligned}\Pi(\tilde{\boldsymbol{q}}, \tilde{\boldsymbol{Q}} = 0) &= \frac{g^2}{2\pi v_z A_3^{2/3}} \int \frac{d^2\boldsymbol{K}}{(2\pi)^2} \int_0^1 dx \left\{ \frac{|\boldsymbol{K}|^6 + x(1-x)(q_0^2 - q_z^2)}{x(1-x)\boldsymbol{q}^2 + |\boldsymbol{K}|^6} - 1 \right\} \\ &= \frac{g^2}{2\pi v_z A_3^{2/3}} \int \frac{d^2\boldsymbol{K}}{(2\pi)^2} \int_0^1 dx \left\{ \frac{-2x(1-x)q_z^2}{x(1-x)\boldsymbol{q}^2 + |\boldsymbol{K}|^6} \right\} \\ &= \frac{g^2}{2\pi v_z A_3^{2/3}} \frac{q_z^2}{|\boldsymbol{q}|^{4/3}} \int_0^1 dx \frac{x^{1/3}(1-x)^{1/3}}{3\sqrt{3}} \\ &= -\frac{g^2}{2\pi v_z A_3^{2/3}} \frac{\Gamma\left(\frac{4}{3}\right)^2}{3\sqrt{3}\Gamma\left(\frac{8}{3}\right)} \frac{q_z^2}{|\boldsymbol{q}|^{4/3}} \\ &= -b_3^{(1)} \frac{g^2}{v_z A_3^{2/3}} \frac{q_z^2}{|\boldsymbol{q}|^{4/3}}.\end{aligned} \tag{5.20}$$

### 5.2 Fermionic self-energy

The first order contribution to the fermionic self-energy is

$$\begin{aligned}\Sigma(k) &= (ig)^2 \int \mathrm{d}q\ G_0(k+q)D(q) \\ &= -g^2 \int \mathrm{d}q \frac{-i(k_0+q_0) + A_3|\boldsymbol{K}+\boldsymbol{Q}|^3[\sigma_1\cos(3\phi_{k+q}) + \sigma_2\sin(3\phi_{k+q})] + v_z(k_z+q_z)\sigma_3}{(k_0+q_0)^2 + A_3^2|\boldsymbol{K}+\boldsymbol{Q}|^6 + v_z^2(k_z+q_z)^2} D(q) \\ &\equiv -\Sigma_0\cdot ik_0 - \Sigma_{12}\cdot A_3|\boldsymbol{K}|^3[\sigma_1\cos(3\phi_k)+\sigma_2\sin(3\phi_k)] - \Sigma_3\cdot v_z k_z\sigma_3 \end{aligned} \tag{5.21}$$

where $D^{-1}(q) = D_0^{-1}(q) - N\Pi(q)$. After absorbing the cutoff-dependent terms in Eq. (5.15) in the counter-terms of the renormalized theory, the dressed bosonic propagator reads

$$D^{-1}(q) = \boldsymbol{Q}^2 + cq_z^2 + b_3^{(1)}\frac{\alpha_N}{v_3^{2/3}}\frac{v_z^2q_z^2}{(q_0^2+v_z^2q_z^2)^{2/3}} - \frac{3\alpha_N}{8\pi^2}\boldsymbol{Q}^2\left(\frac{1}{4}\frac{v_z^2q_z^2}{q_0^2+v_z^2q_z^2} - \ln 2\right). \tag{5.22}$$

To be consistent with the regularization employed in Sec. 5.1, we compute $\Sigma(k)$ by integrating first over $k_0$, then over $k_z$ and finally imposing an in-plane cutoff $\omega < A_3|\boldsymbol{K}|^3 < \Lambda = A_3\Lambda_\perp^3$. Let us define new variables as

$$\begin{cases} A_3^{1/3}Q_x = \rho^{1/3}\cos\theta, \\ A_3^{1/3}Q_y = \rho^{1/3}\sin\theta, \\ v_zq_z = \eta\rho, \\ q_0 = \nu\rho. \end{cases} \tag{5.23}$$

We can then rewrite the propagator as $D^{-1}(q) = A_3^{-2/3}\rho^{2/3}d^{-1}(q)$, where

$$d^{-1}(\rho,\phi,\theta,\nu) = \sin^{2/3}\phi + c\frac{A_3^{2/3}}{v_z^2}\rho^{4/3}\eta^2 + \alpha_N\left[\frac{b_3^{(1)}\eta^2}{(\nu^2+\eta^2)^{2/3}} - \frac{3}{8\pi^2}\left(\frac{1}{4}\frac{\eta^2}{\nu^2+\eta^2} - \ln 2\right)\right]. \tag{5.24}$$

**(i) $\Sigma_0$:**

Here we set $\boldsymbol{K}=0$, $k_z=0$ and expand $G_0(k+q)$ to linear order in $k_0$, which yields

$$\begin{aligned}\Sigma_0 &= g^2\int \mathrm{d}q \frac{q_0^2 - A_3^2\boldsymbol{Q}^6 - v_z^2q_z^2}{(q_0^2+A_3^2\boldsymbol{Q}^6+v_z^2q_z^2)^2}D(q) \\ &= \frac{1}{N(2\pi)^3}\int_\omega^\Lambda \frac{d\rho}{\rho}\int_{-\infty}^{\infty}d\eta\int_{-\infty}^{\infty}d\nu \frac{1}{3}\frac{\nu^2-1-\eta^2}{(\nu^2+1+\eta^2)^2}\left[\frac{b_3^{(1)}\eta^2}{(\nu^2+\eta^2)^{2/3}} - \frac{3}{8\pi^2}\left(\frac{1}{4}\frac{\eta^2}{\nu^2+\eta^2} - \ln 2\right)\right]^{-1} + \mathcal{O}(\alpha_N^{-1}) \\ &= 0.252\frac{\ell}{N} \end{aligned} \tag{5.25}$$

**(ii) $\Sigma_3$:**

Here we set $\boldsymbol{K}=0$, $k_0=0$ and expand $G_0(k+q)$ to linear order in $k_z$, which yields

$$\begin{aligned}\Sigma_3 &= g^2\int \mathrm{d}q \frac{q_0^2 + A_3^2\boldsymbol{Q}^6 - v_z^2q_z^2}{(q_0^2+A_3^2\boldsymbol{Q}^6+v_z^2q_z^2)^2}D(q) \\ &= \frac{1}{N(2\pi)^3}\int_\omega^\Lambda \frac{d\rho}{\rho}\int_{-\infty}^{\infty}d\eta\int_{-\infty}^{\infty}d\nu \frac{1}{3}\frac{\nu^2+1-\eta^2}{(\nu^2+1+\eta^2)^2}\left[\frac{b_3^{(1)}\eta^2}{(\nu^2+\eta^2)^{2/3}} - \frac{3}{8\pi^2}\left(\frac{1}{4}\frac{\eta^2}{\nu^2+\eta^2} - \ln 2\right)\right]^{-1} + \mathcal{O}(\alpha_N^{-1}) \\ &= 0.535\frac{\ell}{N} \end{aligned} \tag{5.26}$$

**(iii) $\Sigma_{12}$:**

Here it is convenient to rewrite the second term in Eq. (5.21) as

$$\Sigma_{12}\cdot A_3|\boldsymbol{K}|^3[\sigma_1\cos(3\phi_k)+\sigma_2\sin(3\phi_k)]\equiv\Sigma_1\cdot A_3(K_x^3-3K_xK_y^2)\sigma_1+\Sigma_2\cdot A_3(K_y^3-3K_x^2K_y)\sigma_2. \tag{5.27}$$

Since rotational symmetry enforces $\Sigma_1=\Sigma_2=\Sigma_{12}$, we show only the computation of $\Sigma_1$. Setting $k_0=0$, $k_z=0$ letting $f(q)$ be the coefficient of $A_3K_x^3\sigma_1$ in the expansion of $G_0(k+q)$ yields

$$\begin{aligned}\Sigma_1&=g^2\int \mathrm{d}q f(q)D(q)\\&=\frac{1}{N(2\pi)^4}\int_\omega^\Lambda\frac{d\rho}{\rho}\int_0^{2\pi}d\theta\int_{-\infty}^{\infty}d\eta\int_{-\infty}^{\infty}d\nu\frac{1}{3}\tilde{f}(\theta,\phi,\nu)\left[\frac{b_3^{(1)}\eta^2}{(\nu^2+\eta^2)^{2/3}}-\frac{3}{8\pi^2}\left(\frac{1}{4}\frac{\eta^2}{\nu^2+\eta^2}-\ln 2\right)\right]^{-1}+\mathcal{O}(\alpha_N^{-1})\\&=0.294\frac{\ell}{N}\end{aligned} \tag{5.28}$$

Therefore, we obtain

$$\gamma_0=\frac{0.252}{N},\quad \gamma_{12}=\frac{0.535}{N},\ \text{and}\ \gamma_3=\frac{0.294}{N}. \tag{5.29}$$

## 5.3 Vertex correction

Finally, we verify that the one-loop correction to the vertex at vanishing external momentum and frequency is consistent with the Ward-Takahashi identity

$$\delta g=(ig)^2\int \mathrm{d}k\ G_0(k)G_0(k)D(k)=g^2\int\frac{d^4k}{(2\pi)^4}\frac{k_0^2-E_k^2}{(k_0^2+E_k^2)^2}D(k)=\Sigma_0=0.252\frac{\ell}{N} \tag{5.30}$$

## 5.4 RG equations

Using the RG equations in Eqs. (2.4)-(2.7), and the form of the counterterms found in this section, we obtain

$$\dot{Z}_\psi(\ell)=-\gamma_0Z_\psi(\ell), \tag{5.31}$$

$$\dot{A}_2(\ell)=(\gamma_{12}-\gamma_0)A_2(\ell), \tag{5.32}$$

$$\dot{v_z}(\ell)=(\gamma_3-\gamma_0)v_z(\ell), \tag{5.33}$$

$$\text{and}\ \dot{\alpha}_N(\ell)=-\frac{3\alpha_N^2(\ell)}{4\pi^2}+\mathcal{O}(1/N), \tag{5.34}$$

with $\gamma_a$ $(a=0,12,3)$ given by Eq. (5.29), and the value of $\delta_a$ $(a=12,3)$ in Eq. (5.17).

Solving these equations we obtain

$$Z_\psi(\ell)=e^{-\gamma_0\ell}, \tag{5.35}$$

$$A_2(\ell)=A_2e^{(\gamma_{12}-\gamma_0)\ell}, \tag{5.36}$$

$$v_z(\ell)=v_ze^{(\gamma_3-\gamma_0)\ell}, \tag{5.37}$$

$$\text{and}\ \alpha_N(\ell)=\frac{\alpha_N^{(0)}}{1+\frac{\alpha_N^{(0)}}{4\pi^2}\ell}. \tag{5.38}$$

# 6 Quadruple Weyl semimetal

We now focus on the quadruple WSM, for which the Hamiltonian (1.1) reads

$$H_4 = A_4 k_\perp^4 [\sigma_1 \cos(4\phi_k) + \sigma_2 \sin(4\phi_k)] + v_z k_z \sigma_3, \tag{6.1}$$

and the energy dispersion is $E_k = \sqrt{A_4^2 |\boldsymbol{K}|^8 + v_z^2 k_z^2}$.

## 6.1 Bosonic self-energy

The polarization bubble contribution for each fermionic species is given by

$$\begin{aligned}\Pi(q) &= g^2 \int \mathrm{d}k \, \mathrm{Tr}\big[G_0(k+q) G_0(k)\big] \\ &= 2g^2 \int \frac{d^4k}{(2\pi)^4} \frac{-k_0(k_0+q_0) + A_4^2 |\boldsymbol{K}|^4 |\boldsymbol{K}+\boldsymbol{Q}|^4 \cos[4(\phi_{k+q} - \phi_k)] + v_z^2 k_z (k_z + q_z)}{[(k_0+q_0)^2 + A_4^2 |\boldsymbol{K}+\boldsymbol{Q}|^8 + v_z^2 (k_z+q_z)^2] \, [k_0^2 + A_4^2 |\boldsymbol{K}|^8 + v_z^2 k_z^2]}. \end{aligned} \tag{6.2}$$

We next make use of Feynman parametrization

$$\frac{1}{ab} = \int_0^1 dx \frac{1}{[xa + (1-x)b]^2} \tag{6.3}$$

and define the scaled momenta $\tilde{\boldsymbol{K}} = A_4^{1/4} \boldsymbol{K}$, $\tilde{k_z} = v_z k_z$, $\tilde{k_0} = k_0$. This yields

$$\Pi(\tilde{q}) = \frac{2g^2}{v_z A_4^{1/2}} \int \frac{d^4k'}{(2\pi)^4} \int_0^1 dx \frac{-k_0'^2 + k_z'^2 + |\boldsymbol{K}|^4 |\boldsymbol{K}+\boldsymbol{Q}|^4 \cos[4(\phi_{k+q} - \phi_k)] + x(1-x)(q_0^2 - q_z^2)}{[k_0'^2 + k_z'^2 + \Delta(x, \boldsymbol{K}, q)]^2}, \tag{6.4}$$

where $k_0' = k_0 + x q_0$, $k_z' = k_z + x q_z$ and $\Delta = x(1-x)(q_0^2 + q_z^2) + x|\boldsymbol{K}+\boldsymbol{Q}|^8 + (1-x)|\boldsymbol{K}|^8$. Following the prescription justified in Sec. 3, we first integrate analytically over the linear directions $k_0$ and $k_z$ to obtain

$$\Pi(\tilde{q}) = \frac{g^2}{2\pi v_z A_4^{1/2}} \int \frac{d^2\boldsymbol{K}}{(2\pi)^2} \int_0^1 dx \left\{ \frac{|\boldsymbol{K}|^4 |\boldsymbol{K}+\boldsymbol{Q}|^4 \cos[4(\phi_{k+q} - \phi_k)] + x(1-x)(q_0^2 - q_z^2)}{x(1-x)\boldsymbol{q}^2 + x|\boldsymbol{K}+\boldsymbol{Q}|^8 + (1-x)|\boldsymbol{K}|^8} - 1 \right\}. \tag{6.5}$$

To proceed with the calculation, we impose a hard UV cutoff $\Lambda_\perp$ in the $\boldsymbol{K}$-space and define adimensional variables $r = \boldsymbol{K}^2/|\boldsymbol{q}|^{1/2}$, $s = \boldsymbol{Q}^2/|\boldsymbol{q}|^{1/2}$ and $\varphi = \tan^{-1}(q_z/q_0)$. If $\theta$ is the angle between $\boldsymbol{K}$ and $\boldsymbol{Q}$, see Fig. 1, using the identity $\cos(4x) = 8\cos^4 x - 8\cos^2 x + 1$ the second term in the numerator can be rewritten as

$$\begin{aligned} |\boldsymbol{K}|^4 |\boldsymbol{K}+\boldsymbol{Q}|^4 \cos\big[4(\phi_{k+q} - \phi_k)\big] &= 8\Big(|\boldsymbol{K}||\boldsymbol{K}+\boldsymbol{Q}| \cos(\phi_{k+q} - \phi_k)\Big)^4 \\ &\quad - 8|\boldsymbol{K}|^2 |\boldsymbol{K}+\boldsymbol{Q}|^2 \Big(|\boldsymbol{K}||\boldsymbol{K}+\boldsymbol{Q}| \cos(\phi_{k+q} - \phi_k)\Big)^2 + |\boldsymbol{K}|^4 |\boldsymbol{K}+\boldsymbol{Q}|^4 \\ &= 8\Big(|\boldsymbol{K}|^2 + |\boldsymbol{K}||\boldsymbol{Q}|\cos\theta\Big)^4 - 8|\boldsymbol{K}|^2 \Big(|\boldsymbol{K}|^2 + |\boldsymbol{Q}|^2 + 2|\boldsymbol{K}||\boldsymbol{Q}|\cos\theta\Big)\Big(|\boldsymbol{K}|^2 + |\boldsymbol{K}||\boldsymbol{Q}|\cos\theta\Big)^2 \\ &\quad + |\boldsymbol{K}|^4 \Big(|\boldsymbol{K}|^2 + |\boldsymbol{Q}|^2 + 2|\boldsymbol{K}||\boldsymbol{Q}|\cos\theta\Big)^2 \\ &= |\boldsymbol{q}|^2 \Big(r^4 + 4r^{7/2}s^{1/2}\cos\theta + 6r^3 s\cos(2\theta) + 4r^{5/2}s^{3/2}\cos(3\theta) + r^2 s^2 \cos(4\theta)\Big). \end{aligned} \tag{6.6}$$

while the integration measure reads

$$\int_{|\boldsymbol{K}|<\Lambda_\perp} \frac{d^2\boldsymbol{K}}{(2\pi)^2} \to \frac{|\boldsymbol{q}|^{1/2}}{2(2\pi)} \int_0^{2\pi} \frac{d\theta}{2\pi} \int_0^{\Lambda_r} dr, \tag{6.7}$$

where $\Lambda_r = \Lambda_\perp^2/|\boldsymbol{q}|^{1/2}$. These changes yield

$$\Pi(\tilde{q}) = \frac{g^2}{8\pi^2 v_z A_4^{1/2}} |\boldsymbol{q}|^{2/3} \int_0^{2\pi} \frac{d\theta}{2\pi} \int_0^{\Lambda_r} dr \underbrace{\int_0^1 dx \left\{ \frac{r^4 + 4r^{7/2}s^{1/2}\cos(\theta) + 6r^3 s\cos(2\theta) + 4r^{5/2}s^{3/2}\cos(3\theta) + r^2s^2\cos(4\theta) + x(1-x)\cos 2\varphi}{x(1-x) + x(r + 2r^{1/2}s^{1/2}\cos\theta + s)^4 + (1-x)r^4} - 1 \right\}}_{h(r,\theta,s,\varphi)} . \tag{6.8}$$

Following the pattern observed for $n = 2$ and $n = 3$, we define a new function

$$f(r,\theta,s,\varphi) = h(r,\theta,s,\varphi) + \frac{16s}{3\sqrt{r^2+1}}, \tag{6.9}$$

which is expected to give a finite result when integrated. Our final expression for $\Pi(\tilde{q})$ reads

$$\begin{aligned} \Pi(\tilde{q}) &= \frac{g^2}{8\pi^2 v_z A_4^{1/2}} |\boldsymbol{q}|^{1/2} \int_0^{2\pi} \frac{d\theta}{2\pi} \int_0^{\Lambda_r} dr \left\{ -\frac{16s}{3\sqrt{r^2+1}} + f(r,\theta,s,\varphi) \right\} \\ &= \frac{g^2}{8\pi^2 v_z A_4^{1/2}} \left[ -\frac{16}{3}\boldsymbol{Q}^2 \sinh^{-1}\left(\frac{\Lambda_\perp^2}{|\boldsymbol{q}|^{1/2}}\right) + |\boldsymbol{q}|^{1/2} F(\Lambda_\perp, s, \varphi) \right], \end{aligned} \tag{6.10}$$

where $F(\Lambda_\perp, s,\varphi) = \int_{-\pi}^{\pi} \frac{d\theta}{2\pi} \int_0^{\Lambda_r} dr f(r,\theta,s,\varphi)$ is UV finite, so we only consider the $\mathcal{O}(\Lambda_\perp^0)$ contribution given by $F_{n=4}(\infty, s, \varphi) \equiv \lim_{\Lambda_\perp\to\infty} F(\Lambda_\perp, s,\varphi)$. Since this integral is analytically intractable, we propose the ansatz

$$F_{n=4}(\infty, s, \varphi) = -8\pi^2 b_4^{(1)} \sin^2\varphi + \frac{16}{3} s \left[ \ln\left(s + \frac{3}{2}\right) + \frac{1}{4}\sin^2\varphi \right], \tag{6.11}$$

where

$$b_4^{(1)} = \frac{\Gamma\left(\frac{5}{4}\right)^2}{6\pi\sqrt{2\pi}} \approx 0.017. \tag{6.12}$$

The ansatz is verified numerically as shown in Fig. 4. We then conclude, using the relation $\sinh^{-1}(z) \approx \ln(2z)$ for $z \gg 1$:

$$\Pi(\tilde{q}) = \frac{g^2}{8\pi^2 v_z A_4^{1/2}} \left[ -8\pi^2 b_4^{(1)} \frac{q_z^2}{|\boldsymbol{q}|^{3/2}} - \frac{16}{3}\boldsymbol{Q}^2 \ln\left(\frac{\Lambda_\perp^2}{|\boldsymbol{q}|^{1/2}}\right) + \frac{16}{3}\boldsymbol{Q}^2 \ln\left(\frac{\boldsymbol{Q}^2}{|\boldsymbol{q}|^{1/2}} + \frac{3}{2}\right) + \frac{16}{3}\boldsymbol{Q}^2 \left(\frac{1}{4}\sin^2\varphi - \ln 2\right) \right]. \tag{6.13}$$

In terms of the unscaled momenta

$$\begin{aligned} \Pi(q) &= -b_4^{(1)} \frac{g^2}{v_z A_4^{1/2}} \frac{v_z^2 q_z^2}{(q_0^2 + v_z^2 q_z^2)^{3/4}} - \frac{2g^2}{3\pi^2 v_z} \boldsymbol{Q}^2 \left[ \ln\left( \frac{A_4^{1/2}\Lambda_\perp^2}{A_4^{1/2}\boldsymbol{Q}^2 + (3/2)(q_0^2 + v_z^2 q_z^2)^{1/4}} \right) - \left(\frac{1}{4}\sin^2\varphi - \ln 2\right) \right] &(6.14) \\ &= -b_4^{(1)} \frac{g^2}{v_z A_4^{1/2}} \frac{v_z^2 q_z^2}{(q_0^2 + v_z^2 q_z^2)^{3/4}} - \frac{2g^2}{3\pi^2 v_z} \boldsymbol{Q}^2 \left[ \ln\left( \frac{\Lambda^{1/2}}{A_4^{1/2}\boldsymbol{Q}^2 + (3/2)(q_0^2 + v_z^2 q_z^2)^{1/4}} \right) - \left(\frac{1}{4}\sin^2\varphi - \ln 2\right) \right]. &(6.15) \end{aligned}$$

Therefore, we obtain

$$\delta_{12} = \frac{\alpha_N}{3\pi^2} \text{ and } \delta_3 = 0. \tag{6.16}$$

Next, we verify that the result given in Eq. (6.14) satisfies the limiting cases (i) $q = 0$, (ii) $\boldsymbol{q} = 0$ and (iii) $\boldsymbol{Q} = 0$.

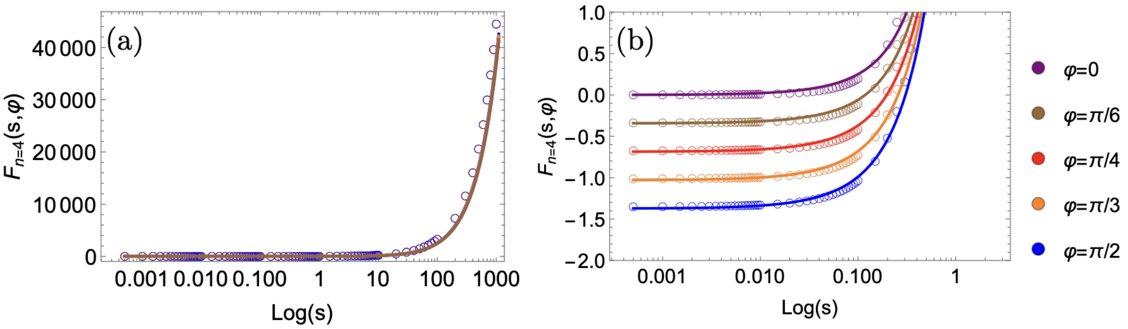


Figure 4: Numerically integrated $F(\Lambda_\perp, s, \varphi)$ (markers) compared to the ansatz $F_{n=4}(\infty, s, \varphi)$ (solid lines) given in Eq. (6.11) for different values of $\varphi$, over (a) a wide range $s \in (10^{-3}, 10^3)$ and (b) small values of $s$.

**(i)** $q = 0$**:**

$$\Pi(\tilde{q} = 0) = 0 \tag{6.17}$$

**(ii)** $\boldsymbol{q} = 0$**:**

$$\begin{aligned}\Pi(\tilde{\boldsymbol{q}} = 0, \tilde{\boldsymbol{Q}}) &= \frac{g^2}{2\pi v_z A_4^{1/2}} \int \frac{d^2\boldsymbol{K}}{(2\pi)^2} \int_0^1 dx \left\{ \frac{|\boldsymbol{K}|^4 |\boldsymbol{K}+\boldsymbol{Q}|^4 \cos[4(\phi_{k+q} - \phi_k)]}{x|\boldsymbol{K}+\boldsymbol{Q}|^8 + (1-x)|\boldsymbol{K}|^8} - 1 \right\} \\ &= -\frac{2g^2}{3\pi^2 v_z} \boldsymbol{Q}^2 \left[ \ln\left(\frac{\Lambda_\perp^2}{\boldsymbol{Q}^2}\right) + \mathcal{O}(1) \right]\end{aligned} \tag{6.18}$$

**(iii)** $\boldsymbol{Q} = 0$**:**

$$\begin{aligned}\Pi(\tilde{\boldsymbol{q}}, \tilde{\boldsymbol{Q}} = 0) &= \frac{g^2}{2\pi v_z A_4^{1/2}} \int \frac{d^2\boldsymbol{K}}{(2\pi)^2} \int_0^1 dx \left\{ \frac{|\boldsymbol{K}|^8 + x(1-x)(q_0^2 - q_z^2)}{x(1-x)\boldsymbol{q}^2 + |\boldsymbol{K}|^8} - 1 \right\} \\ &= \frac{g^2}{2\pi v_z A_4^{1/2}} \int \frac{d^2\boldsymbol{K}}{(2\pi)^2} \int_0^1 dx \left\{ \frac{-2x(1-x)q_z^2}{x(1-x)\boldsymbol{q}^2 + |\boldsymbol{K}|^8} \right\} \\ &= \frac{g^2}{2\pi v_z A_4^{1/2}} \frac{q_z^2}{|\boldsymbol{q}|^{3/2}} \int_0^1 dx \frac{x^{1/4}(1-x)^{1/4}}{4\sqrt{2}} \\ &= -\frac{g^2}{2\pi v_z A_4^{1/2}} \frac{\Gamma\left(\frac{5}{4}\right)^2}{3\sqrt{2\pi}} \frac{q_z^2}{|\boldsymbol{q}|^{3/2}} \\ &= -b_4^{(1)} \frac{g^2}{v_z A_4^{1/2}} \frac{q_z^2}{|\boldsymbol{q}|^{3/2}}.\end{aligned} \tag{6.19}$$

## 6.2 Fermionic self-energy

The first order contribution to the fermionic self-energy is

$$\begin{aligned}\Sigma(k) &= (ig)^2 \int \mathrm{d}q\; G_0(k+q) D(q) \\ &= -g^2 \int \mathrm{d}q \frac{-i(k_0+q_0) + A_4|\boldsymbol{K}+\boldsymbol{Q}|^4[\sigma_1 \cos(4\phi_{k+q}) + \sigma_2 \sin(4\phi_{k+q})] + v_z(k_z+q_z)\sigma_3}{(k_0+q_0)^2 + A_4^2|\boldsymbol{K}+\boldsymbol{Q}|^8 + v_z^2(k_z+q_z)^2} D(q)\end{aligned}$$

$$\equiv -\Sigma_0 \cdot ik_0 - \Sigma_{12} \cdot A_4 |\boldsymbol{K}|^4 [\sigma_1 \cos(4\phi_k) + \sigma_2 \sin(4\phi_k)] - \Sigma_3 \cdot v_z k_z \sigma_3 \tag{6.20}$$

where $D^{-1}(q) = D_0^{-1}(q) - N\Pi(q)$. After absorbing the cutoff-dependent terms in Eq. (6.14) in the counter-terms of the renormalized theory, the dressed bosonic propagator reads

$$D^{-1}(q) = \boldsymbol{Q}^2 + cq_z^2 + b_4^{(1)} \frac{\alpha_N}{A_4^{1/2}} \frac{v_z^2 q_z^2}{(q_0^2 + v_z^2 q_z^2)^{3/4}} - \frac{2\alpha_N}{3\pi^2} \boldsymbol{Q}^2 \left( \frac{1}{4} \frac{v_z^2 q_z^2}{q_0^2 + v_z^2 q_z^2} - \ln 2 \right). \tag{6.21}$$

To be consistent with the regularization employed in Sec. 5.1, we compute $\Sigma(k)$ by integrating first over $k_0$, then over $k_z$ and finally imposing an in-plane cutoff $\omega < A_4|\boldsymbol{K}|^4 < \Lambda = A_4 \Lambda_\perp^4$. Let us define new variables as

$$\begin{cases} A_4^{1/4} Q_x = \rho^{1/4} \cos\theta, \\ A_4^{1/4} Q_y = \rho^{1/4} \sin\theta, \\ v_z q_z = \eta\rho, \\ q_0 = \nu\rho. \end{cases} \tag{6.22}$$

We can then rewrite the propagator as $D^{-1}(q) = A_4^{-1/2} \rho^{1/2} d^{-1}(q)$, where

$$d^{-1}(\rho, \theta, \eta, \nu) = 1 + c\frac{A_4^{1/2}}{v_z^2} \rho^{3/2} \eta^2 + \alpha_N \left[ \frac{b_4^{(1)} \eta^2}{(\nu^2 + \eta^2)^{3/4}} - \frac{2}{3\pi^2} \left( \frac{1}{4} \frac{\eta^2}{\nu^2 + \eta^2} - \ln 2 \right) \right]. \tag{6.23}$$

**(i) $\Sigma_0$:**

Here we set $\boldsymbol{K} = 0$, $k_z = 0$ and expand $G_0(k+q)$ to linear order in $k_0$, which yields

$$\begin{aligned} \Sigma_0 &= g^2 \int \mathrm{d}q \frac{q_0^2 - A_4^2 \boldsymbol{Q}^8 - v_z^2 q_z^2}{(q_0^2 + A_4^2 \boldsymbol{Q}^8 + v_z^2 q_z^2)^2} D(q) \\ &= \frac{1}{N(2\pi)^3} \int_\omega^\Lambda \frac{d\rho}{\rho} \int_{-\infty}^{\infty} d\eta \int_{-\infty}^{\infty} d\nu \frac{1}{4} \frac{\nu^2 - 1 - \eta^2}{(\nu^2 + 1 + \eta^2)^2} \left[ \frac{b_4^{(1)} \eta^2}{(\nu^2 + \eta^2)^{3/4}} - \frac{2}{3\pi^2} \left( \frac{1}{4} \frac{\eta^2}{\nu^2 + \eta^2} - \ln 2 \right) \right]^{-1} + \mathcal{O}(\alpha_N^{-1}) \\ &= 0.165 \frac{\ell}{N} \end{aligned} \tag{6.24}$$

**(ii) $\Sigma_3$:**

Here we set $\boldsymbol{K} = 0$, $k_0 = 0$ and expand $G_0(k+q)$ to linear order in $k_z$, which yields

$$\begin{aligned} \Sigma_3 &= g^2 \int \mathrm{d}q \frac{q_0^2 + A_4^2 \boldsymbol{Q}^8 - v_z^2 q_z^2}{(q_0^2 + A_4^2 \boldsymbol{Q}^8 + v_z^2 q_z^2)^2} D(q) \\ &= \frac{1}{N(2\pi)^3} \int_\omega^\Lambda \frac{d\rho}{\rho} \int_{-\infty}^{\infty} d\eta \int_{-\infty}^{\infty} d\nu \frac{1}{4} \frac{\nu^2 + 1 - \eta^2}{(\nu^2 + 1 + \eta^2)^2} \left[ \frac{b_4^{(1)} \eta^2}{(\nu^2 + \eta^2)^{3/4}} - \frac{2}{3\pi^2} \left( \frac{1}{4} \frac{\eta^2}{\nu^2 + \eta^2} - \ln 2 \right) \right]^{-1} + \mathcal{O}(\alpha_N^{-1}) \\ &= 0.298 \frac{\ell}{N} \end{aligned} \tag{6.25}$$

**(iii) $\Sigma_{12}$:**

Here it is convenient to rewrite the second term in Eq. (6.20) as

$$\Sigma_{12} \cdot A_4 |\boldsymbol{K}|^4 [\sigma_1 \cos(4\phi_k) + \sigma_2 \sin(4\phi_k)] \equiv \Sigma_1 \cdot A_4 (K_x^4 + K_y^4 - 6K_x^2 K_y 2)\sigma_1 + \Sigma_2 \cdot A_4 (4K_x^3 K_y - 4K_x K_y^3)\sigma_2. \tag{6.26}$$

Since rotational symmetry enforces $\Sigma_1 = \Sigma_2 = \Sigma_{12}$, we show only the computation of $\Sigma_1$. Setting $k_0 = 0$, $k_z = 0$ letting $f(q)$ be the coefficient of $A_4 K_x^4 \sigma_1$ in the expansion of $G_0(k+q)$ yields

$$\Sigma_1 = g^2 \int \mathrm{d}q f(q) D(q)$$
$$= \frac{1}{N(2\pi)^4} \int_\omega^\Lambda \frac{d\rho}{\rho} \int_0^{2\pi} d\theta \int_{-\infty}^{\infty} d\eta \int_{-\infty}^{\infty} d\nu \frac{1}{4} \tilde{f}(\theta,\eta,\nu) \left[ \frac{b_3^{(1)} \eta^2}{(\nu^2+\eta^2)^{2/3}} - \frac{3}{8\pi^2} \left( \frac{1}{4} \frac{\eta^2}{\nu^2+\eta^2} - \ln 2 \right) \right]^{-1} + \mathcal{O}(\alpha_N^{-1})$$
$$= 0.263 \frac{\ell}{N} \tag{6.27}$$

Therefore, we obtain

$$\gamma_0 = \frac{0.165}{N}, \quad \gamma_{12} = \frac{0.263}{N} \text{ and } \gamma_3 = \frac{0.298}{N}. \tag{6.28}$$

### 6.3 Vertex correction

Finally, we verify that the one-loop correction to the vertex at vanishing external momentum and frequency is consistent with the Ward-Takahashi identity

$$\delta g = (ig)^2 \int \mathrm{d}k\; G_0(k) G_0(k) D(k) = g^2 \int \frac{d^4 k}{(2\pi)^4} \frac{k_0^2 - E_k^2}{(k_0^2 + E_k^2)^2} D(k) = \Sigma_0 = 0.165 \frac{\ell}{N} \tag{6.29}$$

### 6.4 RG equations

Using the RG equations in Eqs. (2.4)-(2.7), and the form of the counterterms found in this section, we obtain

$$\dot{Z}_\psi(\ell) = -\gamma_0 Z_\psi(\ell), \tag{6.30}$$
$$\dot{A}_2(\ell) = (\gamma_{12} - \gamma_0) A_2(\ell), \tag{6.31}$$
$$\dot{v_z}(\ell) = (\gamma_3 - \gamma_0) v_z(\ell), \tag{6.32}$$
$$\text{and } \dot{\alpha}_N(\ell) = -\frac{4\alpha_N^2(\ell)}{3\pi^2} + \mathcal{O}(1/N), \tag{6.33}$$

with $\gamma_a$ $(a = 0, 12, 3)$ given by Eq. (6.28), and the value of $\delta_a$ $(a = 12, 3)$ in Eq. (6.16).

Solving these equations we obtain

$$Z_\psi(\ell) = e^{-\gamma_0 \ell}, \tag{6.34}$$
$$A_2(\ell) = A_2 e^{(\gamma_{12} - \gamma_0)\ell}, \tag{6.35}$$
$$v_z(\ell) = v_z e^{(\gamma_3 - \gamma_0)\ell}, \tag{6.36}$$
$$\text{and } \alpha_N(\ell) = \frac{\alpha_N^{(0)}}{1 + \frac{\alpha_N^{(0)}}{3\pi^2} \ell}. \tag{6.37}$$

## 7 General Weyl semimetal

We now focus on the general WSM as given in Eq. (1.1), for which the energy dispersion is $E_k = \sqrt{A_n^2 |\boldsymbol{K}|^{2n} + v_z^2 k_z^2}$.

### 7.1 Bosonic self-energy

The polarization bubble contribution for each fermionic species is given by

$$\Pi(q) = g^2 \int \mathrm{d}k\, \mathrm{Tr}\big[ G_0(k+q) G_0(k) \big]$$

$$= 2g^2 \int \frac{d^4k}{(2\pi)^4} \frac{-k_0(k_0+q_0) + A_n^2 |\boldsymbol{K}|^n |\boldsymbol{K}+\boldsymbol{Q}|^n \cos[n(\phi_{k+q}-\phi_k)] + v_z^2 k_z(k_z+q_z)}{[(k_0+q_0)^2 + A_n^2|\boldsymbol{K}+\boldsymbol{Q}|^{2n} + v_z^2(k_z+q_z)^2]\,[k_0^2 + A_n^2|\boldsymbol{K}|^{2n} + v_z^2 k_z^2]}. \tag{7.1}$$

We next make use of Feynman parametrization

$$\frac{1}{ab} = \int_0^1 dx \frac{1}{[xa + (1-x)b]^2} \tag{7.2}$$

and define the scaled momenta $\tilde{\boldsymbol{K}} = A_n^{1/n}\boldsymbol{K}$, $\tilde{k_z} = v_z k_z$, $\tilde{k_0} = k_0$. This yields

$$\Pi(\tilde{q}) = \frac{2g^2}{v_z A_n^{2/n}} \int \frac{d^4k'}{(2\pi)^4} \int_0^1 dx \frac{-k_0'^2 + k_z'^2 + |\boldsymbol{K}|^n|\boldsymbol{K}+\boldsymbol{Q}|^n \cos[n(\phi_{k+q}-\phi_k)] + x(1-x)(q_0^2 - q_z^2)}{\left[k_0'^2 + k_z'^2 + \Delta\,(x,\boldsymbol{K},q)\right]^2}, \tag{7.3}$$

where $k_0' = k_0 + xq_0$, $k_z' = k_z + xq_z$ and $\Delta = x(1-x)(q_0^2+q_z^2) + x|\boldsymbol{K}+\boldsymbol{Q}|^{2n} + (1-x)|\boldsymbol{K}|^{2n}$. Following the prescription justified in Sec. 3, we first integrate analytically over the linear directions $k_0$ and $k_z$ to obtain

$$\Pi(\tilde{q}) = \frac{g^2}{2\pi v_z A_n^{2/n}} \int \frac{d^2\boldsymbol{K}}{(2\pi)^2} \int_0^1 dx \left\{ \frac{|\boldsymbol{K}|^n|\boldsymbol{K}+\boldsymbol{Q}|^n \cos[n(\phi_{k+q}-\phi_k)] + x(1-x)(q_0^2-q_z^2)}{x(1-x)\boldsymbol{q}^2 + x|\boldsymbol{K}+\boldsymbol{Q}|^{2n} + (1-x)|\boldsymbol{K}|^{2n}} - 1 \right\} \tag{7.4}$$

To proceed with the calculation, we impose a hard UV cutoff $\Lambda_\perp$ in the $\boldsymbol{K}$-space and define adimensional variables $r = \boldsymbol{K}^2/|\boldsymbol{q}|^{2/n}$, $s = \boldsymbol{Q}^2/|\boldsymbol{q}|^{2/n}$ and $\varphi = \tan^{-1}(q_z/q_0)$. To deal with the cosine in the numerator, we consider the vectors and angles shown in Fig. 1, which are related by

$$|\boldsymbol{K}+\boldsymbol{Q}||\boldsymbol{K}|\cos[(\phi_{k+q}-\phi_k)] = \boldsymbol{K}\cdot(\boldsymbol{K}+\boldsymbol{Q}) = |\boldsymbol{K}|^2 + |\boldsymbol{Q}||\boldsymbol{K}|\cos\theta, \tag{7.5}$$

where $\theta$ is the angle between $\boldsymbol{K}$ and $\boldsymbol{Q}$, see Fig. 1.

Since the function $\cos(nx)$ can be written in terms of Chebyshev polynomials as $\cos(nx) = T_n(\cos x)$, the first term in the numerator of Eq. (7.4) can be written as

$$|\boldsymbol{K}|^n|\boldsymbol{K}+\boldsymbol{Q}|^n \cos[n(\phi_{k+q}-\phi_k)] = |\boldsymbol{q}|^2\left(r^n + P_n(r,s,\theta)\right), \tag{7.6}$$

where $P_n(r,s,\theta)$ is a polynomial of degree $(2n-1)/2$ in $r$ and we have used the fact that the coefficients of $T_n(x)$ always sum to 1. The polarization then takes the form

$$\Pi(\tilde{q}) = \frac{g^2}{8\pi^2 v_z A_n^{2/n}} |\boldsymbol{q}|^{2/n} \int_0^{\Lambda_r} dr \underbrace{\int_0^{2\pi} \frac{d\theta}{2\pi} \int_0^1 dx \left\{ \frac{r^n + P_n(r,s,\theta) + x(1-x)\cos 2\varphi}{x(1-x) + x(r + 2r^{1/2}s^{1/2}\cos\theta + s)^n + (1-x)r^n} - 1 \right\}}_{h_n(r,s,\varphi)}. \tag{7.7}$$

where $\Lambda_r = \Lambda_\perp^2/|\boldsymbol{q}|^{2/n}$. After integrating over the Feynman parameter $x$ we consistently find that $h_n(r,s,\varphi)$ has the asymptotic behavior

$$h_n(r,s,\varphi) = \begin{cases} \mathcal{O}\left(r^0\right), & \text{for } r \ll 1 \\ -\frac{n^2 s}{3r} + \mathcal{O}\left(r^{-2}\right), & \text{for } r \gg 1 \end{cases}. \tag{7.8}$$

The divergent part can then be extracted by defining

$$f_n(r,s,\varphi) = h_n(r,s,\varphi) + \frac{n^2 s}{3\sqrt{r^2+1}}, \tag{7.9}$$

such that $f_n(r,s,\varphi)$ gives a finite result when integrated. Our final expression for $\Pi(\tilde{q})$ reads

$$\Pi(\tilde{q}) = \frac{g^2}{8\pi^2 v_z A_n^{2/n}} |\boldsymbol{q}|^{2/n} \int_0^{\Lambda_r} dr \left\{ -\frac{n^2 s}{3\sqrt{r^2+1}} + f_n(r,s,\varphi) \right\}$$

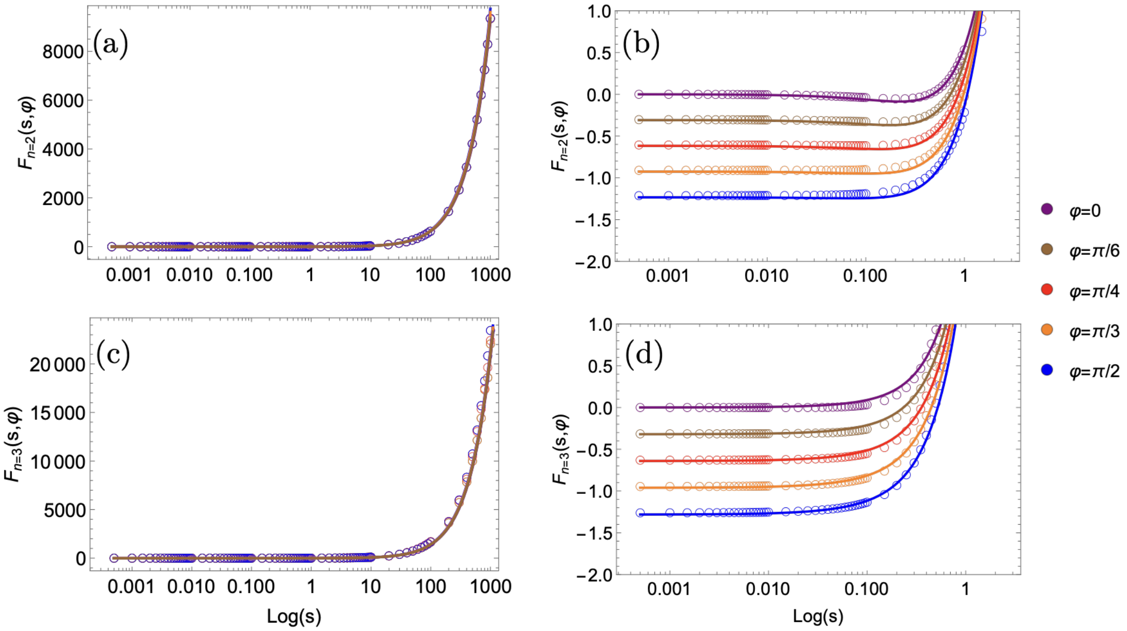


Figure 5: Numerically integrated $F(\Lambda_\perp, s, \varphi)$ (markers) compared to the ansatz $F_n(\infty, s, \varphi)$ (solid lines) for $n = 2$ (upper panel) and $n = 3$ (lower panel).

$$= \frac{g^2}{8\pi^2 v_z A_n^{2/n}} \left[ -\frac{n^2}{2} \boldsymbol{Q}^2 \sinh^{-1}\left( \frac{\Lambda_\perp^2}{|\boldsymbol{q}|^{2/n}} \right) + |\boldsymbol{q}|^{2/n} F_n(\Lambda_\perp, s, \varphi) \right], \tag{7.10}$$

where $F_n(\Lambda_r, s, \varphi) = \int_0^{\Lambda_r} dr f_n(r, s, \varphi)$ is UV finite, so we only consider the $\mathcal{O}(\Lambda_\perp^0)$ contribution given by $F_n(\infty, s, \varphi) \equiv \lim_{\Lambda_\perp \to \infty} F_n(\Lambda_\perp, s, \varphi)$. Since this integral is analytically intractable, we propose the ansatz

$$F_n(\infty, s, \varphi) = -8\pi^2 b_n^{(1)} \sin^2\varphi + \frac{n^2}{3} s \left[ \ln\left( s + b_n^{(2)} \right) + b_n^{(3)} \sin^2\varphi \right], \tag{7.11}$$

where $b_n^{(i)}$, $i = 1, 2, 3$, are real and $n-$dependent, and can be obtained by fitting the ansatz to numerical integration of $f_n(r, s, \varphi)$. For $n = 2$ and $n = 3$ we find:

$$F_{n=2}(\infty, s, \varphi) = -\frac{\pi^2}{8} \sin^2\varphi + \frac{4}{3} s \left[ \ln\left( s + \frac{1}{2} \right) + \frac{2}{5} \sin^2\varphi \right], \tag{7.12}$$

$$\text{and } F_{n=3}(\infty, s, \varphi) = -\frac{4\pi\Gamma\left(\frac{4}{3}\right)^2}{3\sqrt{3}\Gamma\left(\frac{8}{3}\right)} \sin^2\varphi + 3s \left[ \ln\left( s + \frac{5}{4} \right) + \frac{1}{4} \sin^2\varphi \right], \tag{7.13}$$

which are compared to numerical results in Fig. 5.

Using the relation $\sinh^{-1}(z) \approx \ln(2z)$ for $z \gg 1$, we conjecture that the final result for general $n$ takes the form

$$\Pi(\tilde{q}) = -b_n^{(1)} \frac{g^2}{v_z A_n^{2/n}} \frac{q_z^2}{|\boldsymbol{q}|^{2-2/n}} - \frac{g^2}{8\pi^2 v_z A_n^{2/n}} \frac{n^2}{3} \boldsymbol{Q}^2 \left[ \ln\left( \frac{\Lambda_\perp^2}{|\boldsymbol{q}|^{2/n}} \right) - \ln\left( \frac{\boldsymbol{Q}^2}{|\boldsymbol{q}|^{2/n}} + b_n^{(2)} \right) - \left( b_n^{(3)} \sin^2\varphi - \ln 2 \right) \right]. \tag{7.14}$$

In terms of the unscaled momenta, we have

$$\Pi(q) = -b_n^{(1)} \frac{g^2}{v_z A_n^{2/n}} \frac{v_z^2 q_z^2}{(q_0^2 + v_z^2 q_z^2)^{1-1/n}} - \frac{n^2 g^2}{24\pi^2 v_z} \boldsymbol{Q}^2 \left[ \ln\left( \frac{A_n^{2/n} \Lambda_\perp^2}{A_n^{2/n} \boldsymbol{Q}^2 + b_n^{(2)} (q_0^2 + v_z^2 q_z^2)^{1/n}} \right) - \left( b_n^{(3)} \sin^2\varphi - \ln 2 \right) \right], \tag{7.15}$$

$$= -b_n^{(1)} \frac{g^2}{v_z A_n^{2/n}} \frac{v_z^2 q_z^2}{(q_0^2 + v_z^2 q_z^2)^{1-1/n}} - \frac{n^2 g^2}{24\pi^2 v_z} \boldsymbol{Q}^2 \left[ \ln \left( \frac{\Lambda^{2/n}}{A_n^{2/n} \boldsymbol{Q}^2 + b_n^{(2)} (q_0^2 + v_z^2 q_z^2)^{1/n}} \right) - \left( b_n^{(3)} \sin^2 \varphi - \ln 2 \right) \right], \quad (7.16)$$

therefore yielding for the corresponding counterterms,

$$\delta_{12}(\ell) = \frac{n}{12\pi^2} \alpha_N(\ell) \text{ and } \delta_3(\ell) = 0. \quad (7.17)$$

The damping coefficient $b_n^{(1)}$ can be explicitly found by computing $\Pi(q)$ in the limiting case $\boldsymbol{Q} \to 0$

$$\begin{aligned}
\Pi(\tilde{\boldsymbol{q}}, \tilde{\boldsymbol{Q}} = 0) &= \frac{g^2}{2\pi v_z A_n^{2/n}} \int \frac{d^2\boldsymbol{K}}{(2\pi)^2} \int_0^1 dx \left\{ \frac{|\boldsymbol{K}|^{2n} + x(1-x)(q_0^2 - q_z^2)}{x(1-x)\boldsymbol{q}^2 + |\boldsymbol{K}|^{2n}} - 1 \right\} \\
&= \frac{g^2}{2\pi v_z A_n^{2/n}} \int \frac{d^2\boldsymbol{K}}{(2\pi)^2} \int_0^1 dx \frac{-2x(1-x)q_z^2}{x(1-x)\boldsymbol{q}^2 + |\boldsymbol{K}|^{2n}} \\
&= \frac{g^2}{8\pi^2 v_z A_n^{2/n}} \frac{q_z^2}{|\boldsymbol{q}|^{2-2/n}} \int_0^\infty dy \int_0^1 dx \frac{-2x(1-x)}{x(1-x) + y^n} \\
&= -b_n^{(1)} \frac{g^2}{v_z A_n^{2/n}} \frac{q_z^2}{|\boldsymbol{q}|^{2-2/n}}. \quad (7.18)
\end{aligned}$$

Therefore

$$b_n^{(1)} = \frac{1}{8\pi^2} \int_0^\infty dy \int_0^1 dx \frac{2x(1-x)}{x(1-x) + y^n}, \quad (7.19)$$

which is in agreement with Eq. (7.12) and Eq. (7.13), where for $n = 2$ and $n = 3$, we find, respectively

$$b_2^{(1)} = \frac{1}{64}, \text{ and } b_3^{(1)} = \frac{\Gamma\left(\frac{4}{3}\right)^2}{6\pi\sqrt{3}\Gamma\left(\frac{8}{3}\right)}. \quad (7.20)$$

## 7.2 Fermionic self-energy

The first order contribution to the fermionic self-energy is

$$\begin{aligned}
\Sigma(k) &= (ig)^2 \int \mathrm{d}q \; G_0(k+q) D(q) \\
&= -g^2 \int \mathrm{d}q \frac{-i(k_0+q_0) + A_n |\boldsymbol{K}+\boldsymbol{Q}|^n [\sigma_1 \cos(n\phi_{k+q}) + \sigma_2 \sin(n\phi_{k+q})] + v_z(k_z+q_z)\sigma_3}{(k_0+q_0)^2 + A_n^2 |\boldsymbol{K}+\boldsymbol{Q}|^{2n} + v_z^2 (k_z+q_z)^2} D(q) \\
&\equiv -\Sigma_0 \cdot ik_0 - \Sigma_{12} \cdot A_n |\boldsymbol{K}|^n [\sigma_1 \cos(n\phi_k) + \sigma_2 \sin(n\phi_k)] - \Sigma_3 \cdot v_z k_z \sigma_3 \quad (7.21)
\end{aligned}$$

where $D^{-1}(q) = D_0^{-1}(q) - N\Pi(q)$. After absorbing the cutoff-dependent terms in Eq. (7.15) in the counter-terms of the renormalized theory, the dressed bosonic propagator reads

$$D^{-1}(q) = \boldsymbol{Q}^2 + cq_z^2 + b_n^{(1)} \frac{\alpha_N}{A_n^{2/n}} \frac{v_z^2 q_z^2}{(q_0^2 + v_z^2 q_z^2)^{1-1/n}} - \frac{n^2 \alpha_N}{24\pi^2} \boldsymbol{Q}^2 \left( b_n^{(3)} \frac{v_z^2 q_z^2}{q_0^2 + v_z^2 q_z^2} - \ln 2 \right). \quad (7.22)$$

To be consistent with the reularization employed in Sec. 7.1, we compute $\Sigma(k)$ by integrating first over $k_0$, then over $k_z$ and finally imposing an in-plane cutoff $\omega < A_n |\boldsymbol{K}|^n < \Lambda = A_n \Lambda_\perp^n$. Let us define new variables by

$$\begin{cases}
A_n^{1/n} Q_x = \rho^{1/n} \cos\theta, \\
A_n^{1/n} Q_y = \rho^{1/n} \sin\theta, \\
v_z q_z = \eta\rho, \\
q_0 = \nu\rho.
\end{cases} \quad (7.23)$$

We can then rewrite the propagator as $D^{-1}(q) = A_n^{-2/n}\rho^{2/n}d^{-1}(q)$, where

$$d^{-1}(\rho,\phi,\theta,\nu) = \sin^{2/n}\phi + c\frac{A_n^{2/n}}{v_z^2}\rho^{2-2/n}\eta^2 + \alpha_N\left[\frac{b_n^{(1)}\eta^2}{(\nu^2+\eta^2)^{1-1/n}} - \frac{n^2}{24\pi^2}\left(b_n^{(3)}\frac{\eta^2}{\nu^2+\eta^2} - \ln 2\right)\right]. \tag{7.24}$$

Using the Jacobian of the transformation

$$\frac{\partial(q_0,q_x,q_y,q_z)}{\partial(\rho,\phi,\theta,\nu)} = \frac{\rho^{1+2/n}}{nv_zA_n^{2/n}}, \tag{7.25}$$

we separately compute the coefficients in Eq. (7.21) as follows.

**(i) $\Sigma_0$:**

Here we set $\boldsymbol{K}=0$, $k_z=0$ and expand $G_0(k+q)$ to linear order in $k_0$, which yields

$$\begin{aligned}\Sigma_0 &= g^2\int \mathrm{d}q\frac{q_0^2 - A_n^2\boldsymbol{Q}^{2n} - v_z^2q_z^2}{(q_0^2 + A_n^2\boldsymbol{Q}^{2n} + v_z^2q_z^2)^2}D(q)\\ &= \int_\omega^\Lambda\frac{d\rho}{\rho}\int_{-\infty}^{\infty}d\eta\int_{-\infty}^{\infty}d\nu\frac{1}{N(2\pi)^3}\frac{1}{n}\frac{\nu^2-1-\eta^2}{(\nu^2+1+\eta^2)^2}\left[\frac{b_n^{(1)}\eta^2}{(\nu^2+\eta^2)^{1-1/n}} - \frac{n^2}{24\pi^2}\left(b_n^{(3)}\frac{\eta^2}{\nu^2+\eta^2}-\ln 2\right)\right]^{-1} + \mathcal{O}(\alpha_N^{-1})\\ &= \gamma_0\ \ell \end{aligned}\tag{7.26}$$

**(ii) $\Sigma_3$:**

Here we set $\boldsymbol{K}=0$, $k_0=0$ and expand $G_0(k+q)$ to linear order in $k_z$, which yields

$$\begin{aligned}\Sigma_3 &= g^2\int \mathrm{d}q\frac{q_0^2 + A_n^2\boldsymbol{Q}^{2n} - v_z^2q_z^2}{(q_0^2 + A_n^2\boldsymbol{Q}^{2n} + v_z^2q_z^2)^2}D(q)\\ &= \int_\omega^\Lambda\frac{d\rho}{\rho}\int_{-\infty}^{\infty}d\eta\int_{-\infty}^{\infty}d\nu\frac{1}{N(2\pi)^3}\frac{1}{n}\frac{\nu^2+1-\eta^2}{(\nu^2+1+\eta^2)^2}\left[\frac{b_n^{(1)}\eta^2}{(\nu^2+\eta^2)^{1-1/n}} - \frac{n^2}{24\pi^2}\left(b_n^{(3)}\frac{\eta^2}{\nu^2+\eta^2}-\ln 2\right)\right]^{-1} + \mathcal{O}(\alpha_N^{-1})\\ &= \gamma_3\ \ell \end{aligned}\tag{7.27}$$

**(iii) $\Sigma_{12}$:**

Here it is convenient to rewrite the second term in Eq. (7.21) in cartesian coordinates. Explicitly, for $n=2$ and $n=3$

$$\Sigma_{12}\cdot A_2|\boldsymbol{K}|^2[\sigma_1\cos(2\phi_k)+\sigma_2\sin(2\phi_k)] \equiv \Sigma_1\cdot A_2(K_x^2-K_y^2)\sigma_1 + \Sigma_2\cdot A_2 2K_xK_y\sigma_2, \tag{7.28}$$

$$\Sigma_{12}\cdot A_3|\boldsymbol{K}|^3[\sigma_1\cos(3\phi_k)+\sigma_2\sin(3\phi_k)] \equiv \Sigma_1\cdot A_3(K_x^3-3K_xK_y^2)\sigma_1 + \Sigma_2\cdot A_3(K_y^3-3K_x^2K_y)\sigma_2. \tag{7.29}$$

Since rotational symmetry enforces $\Sigma_1=\Sigma_2=\Sigma_{12}$, we can compute only $\Sigma_1$ by setting $k_0=k_z=0$ and taking the coefficient of $A_nK_x^n\sigma_1$ in the expansion of $G_0(k+q)$, which we call $g_n$. This yields an integral of the form

$$\begin{aligned}\Sigma_1 &= g^2\int \mathrm{d}q\frac{q_0^2 + A_n^2\boldsymbol{Q}^{2n} - v_z^2q_z^2}{(q_0^2 + A_n^2\boldsymbol{Q}^{2n} + v_z^2q_z^2)^2}D(q)\\ &= \int_\omega^\Lambda\frac{d\rho}{\rho}\int_0^{2\pi}d\theta\int_{-\infty}^{\infty}d\eta\int_{-\infty}^{\infty}d\nu\frac{1}{N(2\pi)^4}\frac{1}{n}g_n(\rho,\phi,\theta,\nu)\left[\frac{b_n^{(1)}\eta^2}{(\nu^2+\eta^2)^{1-1/n}} - \frac{n^2}{24\pi^2}\left(b_n^{(3)}\frac{\eta^2}{\nu^2+\eta^2}-\ln 2\right)\right]^{-1} + \mathcal{O}(\alpha_N^{-1})\\ &= \gamma_{12}\ \ell \end{aligned}\tag{7.30}$$

Therefore, the coefficients $\gamma_0$, $\gamma_{12}$ and $\gamma_3$ are independent of $\ell$ and can obtained by integrating numerically over $\phi, \theta$ and $\nu$. The results for $n=1,2,3,4$ and conjectures for general $n$ are summarized in Table 1.

| CC | $n=1$ | $n=2$ | $n=3$ | $n=4$ | general $n>1$ |
|---|---|---|---|---|---|
| $\gamma_0$ | 0 | $0.344/N$ | $0.252/N$ | $0.165/N$ | Eq. (7.26) |
| $\gamma_{12}$ | $2.4/N$ | $0.747/N$ | $0.294/N$ | $0.263/N$ | Eq. (7.30) |
| $\gamma_3$ | $2.4/N$ | $1.172/N$ | $0.535/N$ | $0.298/N$ | Eq. (7.27) |
| $\delta_{12}$ | $\alpha_N/12\pi^2$ | $\alpha_N/6\pi^2$ | $\alpha_N/4\pi^2$ | $\alpha_N/3\pi^2$ | $n\,\alpha_N/12\pi^2$ |
| $\delta_3$ | $v_z^2\alpha_N/(12\pi^2 A_1^2)$ | 0 | 0 | 0 | 0 |

Table 1: Values of the one-loop counterterm (CC) coefficients for different values of the monopole charge $n$.

### 7.3 Vertex correction

Finally, we verify that the one-loop correction to the vertex at vanishing external momentum and frequency is consistent with the Ward-Takahashi identity

$$\delta g = (ig)^2 \int \mathrm{d}k\ G_0(k)G_0(k)D(k) = g^2 \int \frac{d^4k}{(2\pi)^4} \frac{k_0^2 - E_k^2}{\left(k_0^2 + E_k^2\right)^2} D(k) = \Sigma_0 \tag{7.31}$$

### 7.4 RG equations

Using the RG equations in Eqs. (2.4)-(2.7), and we now write the $\beta$ functions for a general $n > 1$, which take the form

$$\dot{Z}_\psi(\ell) = -\gamma_0 Z_\psi(\ell), \tag{7.32}$$

$$\dot{A}_2(\ell) = (\gamma_{12} - \gamma_0) A_2(\ell), \tag{7.33}$$

$$\dot{v_z}(\ell) = (\gamma_3 - \gamma_0) v_z(\ell), \tag{7.34}$$

$$\text{and } \dot{\alpha}_N(\ell) = -\frac{n\alpha_N^2(\ell)}{12\pi^2} + \mathcal{O}(1/N), \tag{7.35}$$

with $\gamma_a$, $a = 0, 12, 3$, respectively given by Eqs. (7.26), (7.30), and(7.27), while the values of $\delta_a$ $(a = 12, 3)$ are given in Eq. (7.17).

Solving the RG flow equations, we obtain

$$Z_\psi(\ell) = e^{-\gamma_0 \ell}, \tag{7.36}$$

$$A_2(\ell) = A_2 e^{(\gamma_{12} - \gamma_0)\ell}, \tag{7.37}$$

$$v_z(\ell) = v_z e^{(\gamma_3 - \gamma_0)\ell}, \tag{7.38}$$

$$\text{and } \alpha_N(\ell) = \frac{\alpha_N^{(0)}}{1 + \frac{n\alpha_N^{(0)}}{12\pi^2}\ell}. \tag{7.39}$$

# 8 Real-space form of the dressed Coulomb interaction and anisotropic screening

The (static) interaction between two test charges is obtained by Fourier transforming the *dressed* Coulomb propagator. Therefore, once the bare kernel is renormalized by the polarization $\Pi(q)$ and by the RG running of parameters, the effective Coulomb law becomes *scale dependent* and generically *anisotropic*. Concretely, evaluated at an external scale $E$ (with RG "time" $\ell_E \equiv \ln(\Lambda/E)$), we define

$$V_E(\boldsymbol{r}) \;\propto\; g^2(E)\int \frac{d^2q_\perp\, dq_z}{(2\pi)^3}\,\frac{e^{i\boldsymbol{q}_\perp\cdot\boldsymbol{r}_\perp + iq_z z}}{D_E^{-1}(\boldsymbol{q}_\perp, q_z)}\,, \tag{8.1}$$

where $D_E^{-1}$ is the static dressed kernel evaluated at $\ell = \ell_E$.

## 8.1 Irrelevance of quadratic anisotropic term in the Coulomb propagator

Consider the analytic quadratic term in the bare Coulomb propagator

$$D_0^{-1}(\boldsymbol{q}_\perp, q_z) = a_\perp(E)\, q_\perp^2 + c(E)\, q_z^2. \tag{8.2}$$

We will show that for higher- charge Weyl points ($n > 1$) the *quadratic* longitudinal operator $q_z^2$ is *irrelevant* by simple power counting. Indeed, under the anisotropic scaling appropriate for $E_{\boldsymbol{k}} \sim \sqrt{A_n^2 k_\perp^{2n} + v_z^2 k_z^2}$,

$$q_\perp \to e^{-\ell/n} q_\perp, \qquad q_z \to e^{-\ell} q_z, \tag{8.3}$$

so that

$$q_\perp^2 \to e^{-2\ell/n} q_\perp^2, \qquad q_z^2 \to e^{-2\ell} q_z^2, \tag{8.4}$$

and therefore $q_z^2$ decays parametrically faster than $q_\perp^2$ for any $n > 1$. Equivalently, if one normalizes the kernel by keeping the transverse piece $q_\perp^2$ fixed, the coefficient of the quadratic longitudinal term has negative engineering dimension,

$$c \;\to\; c\, e^{-2(1-1/n)\ell}, \qquad \Rightarrow \qquad \dot{c} = -2\Big(1 - \frac{1}{n}\Big)c, \tag{8.5}$$

showing that the $q_z^2$ structure is irrelevant already at tree level for $n > 1$. Consequently, at sufficiently long wavelengths the longitudinal dependence of the dressed kernel is not controlled by $q_z^2$, but rather by the nonanalytic $|q_z|^{2/n}$ term generated by the fermionic bubble (discussed next).

## 8.2 Nonanalytic longitudinal screening and real-space form of the dressed interaction for $n > 1$

For generalized Weyl nodes ($n > 1$), the one-loop polarization bubble contains besides the transverse $q_\perp^2$ contribution, a finite (non-UV-divergent) bubble-generated *nonanalytic* longitudinal term. In the static limit, the longitudinal term in Eq. (7.15) reduces to

$$\Pi_z(0, q_z) \;=\; -\,\kappa_n\,\frac{g^2}{A_n^{2/n}}\,v_z^{\frac{2}{n}-1}\,|q_z|^{2/n}, \qquad \kappa_n \equiv b_n^{(1)}. \tag{8.6}$$

Since at tree level $q_\perp \to e^{-\ell/n} q_\perp$ and $q_z \to e^{-\ell} q_z$, one has $q_\perp^2 \sim e^{-2\ell/n}$ and $|q_z|^{2/n} \sim e^{-2\ell/n}$, while $q_z^2 \sim e^{-2\ell}$ is more irrelevant for any $n > 1$. Therefore, we can drop the quadratic $q_z^2$ piece, and the (static) dressed Coulomb kernel at an external scale $E$ (with $\ell_E = \ln(\Lambda/E)$) can be written as

$$D_E^{-1}(\boldsymbol{q}_\perp, q_z) \;\simeq\; a_\perp(E)\, q_\perp^2 \;+\; a_z(E)\, |q_z|^{2/n}, \tag{8.7}$$

where $a_z(E)$ collects the finite coefficient generated by the bubble [Eq. (8.6)]. Equation (8.7) makes explicit that the interaction remains long-ranged (no mass term), but becomes anisotropic.

**Form of the potential in real space.** The static interaction is obtained by Fourier transforming the dressed propagator,

$$V_E(\boldsymbol{r}_\perp, z) \;\propto\; g^2(E) \int \frac{d^2 q_\perp \, dq_z}{(2\pi)^3} \, \frac{e^{i\boldsymbol{q}_\perp \cdot \boldsymbol{r}_\perp + i q_z z}}{a_\perp(E)\, q_\perp^2 + a_z(E)\, |q_z|^{2/n}}. \tag{8.8}$$

Performing the transverse integral first yields the representation

$$V_E(\boldsymbol{r}_\perp, z) \;\propto\; \frac{g^2(E)}{4\pi^2 \, a_\perp(E)} \int_{-\infty}^{\infty} dq_z \; e^{i q_z z} \; K_0\Big(\xi(E)\, r_\perp \, |q_z|^{1/n}\Big), \qquad \xi(E) \equiv \sqrt{\frac{a_z(E)}{a_\perp(E)}}\,, \tag{8.9}$$

with $K_0$ the modified Bessel function. Rescaling $t = |q_z|\,|z|$ then gives the anisotropic scaling form

$$V_E(\boldsymbol{r}_\perp, z) \;\propto\; \frac{g^2(E)}{a_\perp(E)} \, \frac{1}{|z|} \; F_n\bigg(\xi(E)\, \frac{r_\perp}{|z|^{1/n}}\bigg)\,, \tag{8.10}$$

where the dimensionless scaling function can be written as

$$F_n(x) \equiv \frac{1}{2\pi^2} \int_0^\infty dt \;\cos t \; K_0\big(x\, t^{1/n}\big). \tag{8.11}$$

This form also clarifies the terminology used in the main text: "transverse logarithmic dressing" refers to the dominant RG renormalization of the $q_\perp^2$ coefficient (encoded in $a_\perp$), while the nonanalytic longitudinal term $|q_z|^{2/n}$ ensures a nontrivial $z$-dependence even though the quadratic $q_z^2$ is irrelevant.

**In-plane potential ($z = 0$).** Setting $z = 0$ in Eq. (8.8) gives

$$V_E(r_\perp, 0) \;\propto\; g^2(E) \int \frac{d^2 q_\perp}{(2\pi)^2} \, e^{i\boldsymbol{q}_\perp \cdot \boldsymbol{r}_\perp} \int \frac{dq_z}{2\pi} \, \frac{1}{a_\perp(E)\, q_\perp^2 + a_z(E)\, |q_z|^{2/n}}. \tag{8.12}$$

To extract the long-distance tail, rescale $q_z = q_\perp^n t$, which yields a $q_\perp^{n-2}$ dependence from the $q_z$-integration. The remaining dimensionless $t$-integral contains an $r_\perp$-independent UV piece that contributes only short-range contact terms, while the long-distance behavior follows from the $q_\perp^{n-2}$ scaling. One finds

$$V_E(r_\perp, 0) \;\sim\; g^2(E)\, a_\perp(E)^{\frac{n}{2}-1} \big[a_z(E)\big]^{-\frac{n}{2}} \, \frac{C_n}{r_\perp^n}, \qquad (n > 1), \tag{8.13}$$

with $C_n > 0$ an $n$-dependent constant. Thus, the bubble-induced $|q_z|^{2/n}$ term induces a fast-decaying in-plane tail $V_E(r_\perp, 0) \propto r_\perp^{-n}$. We notice that the real-space interaction inherits RG running through $g(E)$, $a_\perp(E)$, and $a_z(E)$ evaluated at the matching scale $\ell_E = \ln(\Lambda/E)$.

# 9 Logarithmic corrections to observables

Here we derive the explicit multiplicative logarithmic corrections quoted in the main text for thermodynamic observables (specific heat and compressibility) and transport (optical conductivity), using the fact that the Coulomb coupling is marginally irrelevant and therefore runs as $\alpha_{_N}(E) \sim 1/\ln(\Lambda/E)$ at low energies. To this end, we first obtain the explicit form of the renormalized (RG-improved) fermion Green's function and (for completeness) the form of the running effective structure constant.

## 9.1 Renormalized fermion Green's function from the Callan–Symanzik equation

The renormalized fermion two-point function is obtained by solving the Callan–Symanzik (CS) equation for the Green's function $G(\omega, \boldsymbol{k})$ [4]. After integrating out an infinitesimal Wilsonian shell and rescaling back to the original cutoff, $G$ obeys the CS equation

$$\left[\frac{\partial}{\partial \ell} + \beta_{\alpha_N} \frac{\partial}{\partial \alpha_{_N}} + \beta_A \frac{\partial}{\partial A_n} + \beta_v \frac{\partial}{\partial v_z} + \beta_c \frac{\partial}{\partial c} - \gamma_\psi(\ell)\right] G(\omega, \boldsymbol{k}; \ell) = 0, \tag{9.1}$$

where $\ell$ is the RG parameter, $\beta_X \equiv dX/d\ell$ are the beta functions for the running parameters $X \in \{\alpha_{_N}, A_n, v_z, c\}$, and the fermion-field anomalous dimension is

$$\gamma_\psi(\ell) \equiv -\frac{d \ln Z_\psi(\ell)}{d\ell}. \tag{9.2}$$

With our conventions, $\gamma_\psi(\ell)$ coincides with the frequency anomalous dimension extracted from the $i\omega$ component of the one-loop self-energy, i.e. $\gamma_\psi(\ell) = \gamma_0(\ell)$.

Equation (9.1) is solved by the method of characteristics. Using the anisotropic rescaling appropriate to the generalized Weyl dispersion,

$$\omega \to \omega e^{\ell}, \qquad k_z \to k_z e^{\ell}, \qquad k_\perp \to k_\perp e^{\ell/n}, \tag{9.3}$$

(which ensures that $\omega$, $v_z k_z$, and $A_n k_\perp^n$ scale identically), one finds

$$G(\omega, \boldsymbol{k}) = \exp\left[-\int_0^{\ell} d\ell' \, \gamma_\psi(\ell')\right] G\Big(\omega e^{\ell},\, k_z e^{\ell},\, k_\perp e^{\ell/n};\, \alpha_{_N}(\ell), A_n(\ell), v_z(\ell), c(\ell)\Big). \tag{9.4}$$

To resum the leading logarithms one chooses $\ell$ to match the external scale, so that the residual Green's function on the right-hand side is evaluated at order-one dimensionless arguments. A convenient matching choice is

$$\ell \simeq \ln\left(\frac{\Lambda}{\max\{|\omega|,\, E_{\boldsymbol{k}}\}}\right) \text{ with } E_{\boldsymbol{k}} \equiv \sqrt{A_n^2 k_\perp^{2n} + v_z^2 k_z^2}, \tag{9.5}$$

with $\Lambda$ the UV scale of the low-energy theory. Approximating the remaining Green's function in Eq. (9.4) by its tree-level form but evaluated at the running couplings then yields the standard RG-improved propagator,

$$G(\omega, \boldsymbol{k}) \sim \frac{Z_\psi(\ell)}{i\omega - A_n(\ell)\, k_\perp^n\, \boldsymbol{\sigma}\cdot\hat{\boldsymbol{n}}_k - v_z(\ell)\, k_z\, \sigma_3}, \text{ where } Z_\psi(\ell) \equiv \exp\left[-\int_0^{\ell} d\ell' \, \gamma_\psi(\ell')\right], \tag{9.6}$$

which is the form quoted in the main text. The scale dependence thus enters exclusively through (i) the wave-function factor governed by the fermion anomalous dimension and (ii) the running band parameters evaluated at the matching scale in Eq. (9.5). In particular, when $\alpha_{_N}(\ell)$ is marginally irrelevant and runs only logarithmically, the RG flow of $Z_\psi(\ell)$ and of $A_n(\ell), v_z(\ell)$ is parametrically slow, producing a broad crossover with gradually suppressed spectral weight and anisotropic broadening of single-particle spectral features.

## 9.2 Running effective fine structure constant coupling

For $n > 1$ the one-loop transverse polarization yields

$$\delta_{12} = \frac{d\Pi_{12}}{d\ell} = \bar{\delta}_{12}\, \alpha_{_N}(\ell), \qquad \bar{\delta}_{12} \equiv \frac{n}{12\pi^2}, \tag{9.7}$$

and $\delta_3 = 0$. Using the RG equation $\dot{g} = -(\delta_{12}/2)g$ gives

$$\frac{dg^2}{d\ell} = -\delta_{12}\, g^2 = -\bar{\delta}_{12}\, \alpha_{_N}\, g^2. \tag{9.8}$$

In the infrared, the leading flow of $\alpha_{_N} \equiv N g^2/v_z$ is dominated by the $\delta_{12}$ term (velocity renormalization contributes only at subleading order in $\alpha_{_N}$), so we obtain

$$\frac{d\alpha_{_N}}{d\ell} = -\bar{\delta}_{12}\, \alpha_{_N}^2 + \mathcal{O}\left(\frac{\alpha_{_N}^2}{N}\right). \tag{9.9}$$

Solving Eq. (9.9) gives

$$\alpha_{_N}(\ell) = \frac{\alpha_{_N}^{(0)}}{1 + \bar{\delta}_{12}\, \alpha_{_N}^{(0)}\, \ell}, \qquad \ell_E \equiv \ln\frac{\Lambda}{E}, \tag{9.10}$$

or, equivalently, at the external scale $E = \max\{T, \omega\}$,

$$\alpha_{_N}(E) = \frac{\alpha^0_{_N}}{L_E}, \tag{9.11}$$

with $L_E \equiv 1 + \bar{\delta}_{12}\,\alpha^0_{_N}\ \ln\frac{\Lambda}{E}$ and $\alpha^0_{_N}$ the bare fine structure constant. In the same regime the anomalous dimensions are linear in $\alpha_{_N}$,

$$\gamma_i(\ell) \equiv \frac{d\Sigma_i}{d\ell} \simeq \frac{\bar{\gamma}_i}{N}\,\alpha_{_N}(\ell), \qquad \text{for } i = 0, 12, 3, \tag{9.12}$$

where $\bar{\gamma}_i$ are numerical constants fixed by the dressed-boson one-loop integrals (for their explicit integral representations and the numerical values for $n = 2, 3,$ and 4, see Table 1).

Using $d\ln Z_\psi/d\ell = -\gamma_0$ and $d\ln A_n/d\ell = \gamma_{12} - \gamma_0$, $d\ln v_z/d\ell = \gamma_3 - \gamma_0$, we find

$$Z_\psi(E) = \exp\Big[-\int_0^{\ell_E} d\ell\,\gamma_0(\ell)\Big] \simeq L_E^{-\eta_\psi}, \tag{9.13}$$

$$A_n(E) = A_n\ \exp\Big[\int_0^{\ell_E} d\ell\,(\gamma_{12} - \gamma_0)\Big] \simeq A_n\, L_E^{\eta_A}, \tag{9.14}$$

$$\text{and } v_z(E) = v_z\ \exp\Big[\int_0^{\ell_E} d\ell\,(\gamma_3 - \gamma_0)\Big] \simeq v_z\, L_E^{\eta_v}, \tag{9.15}$$

with the scaling exponents

$$\eta_\psi = \frac{\bar{\gamma}_0}{\bar{\delta}_{12}N}, \qquad \eta_A = \frac{\bar{\gamma}_{12} - \bar{\gamma}_0}{\bar{\delta}_{12}N} \text{ and } \eta_v = \frac{\bar{\gamma}_3 - \bar{\gamma}_0}{\bar{\delta}_{12}N}. \tag{9.16}$$

As $E \to 0$, $L_E \sim \ln(\Lambda/E)$ and Eqs. (9.13)–(9.15) become pure powers of $\ln(\Lambda/E)$.

## 9.3 Density of states with logarithmic corrections

For the dispersion $E_{\boldsymbol{k}} = \sqrt{A_n^2 k_\perp^{2n} + v_z^2 k_z^2}$, the noninteracting DOS scales as $\rho_0(E) \propto E^{2/n}/(v_z A_n^{2/n})$. A convenient explicit derivation starts from

$$\rho_0(E) = \int \frac{d^3k}{(2\pi)^3}\,\delta\Big(E - \sqrt{A_n^2 k_\perp^{2n} + v_z^2 k_z^2}\Big), \tag{9.17}$$

and uses cylindrical coordinates $d^3k = k_\perp\, dk_\perp\, d\phi\, dk_z$ to integrate over $k_z$:

$$\int_{-\infty}^{\infty} dk_z\ \delta\Big(E - \sqrt{A_n^2 k_\perp^{2n} + v_z^2 k_z^2}\Big) = \frac{2E}{v_z\sqrt{E^2 - A_n^2 k_\perp^{2n}}}\,\Theta\big(E - A_n k_\perp^n\big). \tag{9.18}$$

Performing the remaining $k_\perp$ integral with the substitution $t = A_n k_\perp^n/E$ yields the scaling form

$$\rho_0(E) = \frac{C_n}{v_z\, A_n^{2/n}}\, E^{2/n}, \tag{9.19}$$

where $C_n$ is a positive $n$-dependent constant (an order-one Beta-function factor not needed for the scaling).

Including the RG-improved renormalizations, we take the interacting DOS to inherit the multiplicative wave-function factor and the running band parameters,

$$\rho(E) \sim Z_\psi(E)\,\frac{E^{2/n}}{v_z(E)\,A_n(E)^{2/n}}, \tag{9.20}$$

implying that

$$\rho(E) \sim \frac{E^{2/n}}{v_z\, A_n^{2/n}}\, L_E^{-p_\rho}, \tag{9.21}$$

with

$$p_\rho = \eta_\psi + \eta_v + \frac{2}{n}\,\eta_A. \tag{9.22}$$

### 9.4 Specific heat and compressibility

The internal energy density scales as $u(T) \sim \int dE\, E\, \rho(E)\, f(E/T)$, where $f$ is the Fermi function. Using Eq. (9.20) and scaling $E = Tx$, the logarithm varies slowly over the thermal window and can be taken at $E \sim T$ to leading-log accuracy, giving

$$u(T) \sim T^{2+2/n}\, L_T^{-p_\rho}, \text{ where } L_T \equiv 1 + \bar{\delta}_{12}\alpha_N^{(0)} \ln\frac{\Lambda}{T}. \tag{9.23}$$

Therefore the specific heat $C(T) = du/dT$ becomes

$$C(T) \sim T^{1+2/n}\, L_T^{-p_{\rm th}}, \tag{9.24}$$

with $p_{\rm th} = p_\rho = \eta_\psi + \eta_v + \frac{2}{n}\,\eta_A$. The compressibility at charge neutrality can be written as

$$\kappa(T) = \frac{\partial n}{\partial \mu}\bigg|_{\mu=0} = \int_0^\infty dE\, \rho(E) \left(-\frac{\partial f(E/T)}{\partial E}\right), \tag{9.25}$$

which similarly for $E \sim T$ yields

$$\kappa(T) \sim T^{2/n}\, L_T^{-p_{\rm th}}. \tag{9.26}$$

### 9.5 Optical conductivity and its logarithmic corrections

We begin with the Kubo formula for the optical conductivity in terms of the current–current correlator,

$$\sigma_{ij}(\omega) = \frac{1}{\omega} \lim_{\epsilon\to 0} \text{Im}\, \Pi_{ij}(i\Omega \to \omega + i\epsilon, \boldsymbol{q} = 0), \tag{9.27}$$

where the polarization tensor is

$$\Pi_{ij}(i\Omega) = -\int \frac{d^3k}{(2\pi)^3} \int \frac{d\omega}{2\pi}\, \text{Tr}\Big[j_i(\boldsymbol{k})\, G(\boldsymbol{k}, i\omega)\, j_j(\boldsymbol{k})\, G(\boldsymbol{k}, i\omega + i\Omega)\Big]. \tag{9.28}$$

Here $j_i = \partial H/\partial k_i$ is the current operator in the $i$th direction and $G$ is the fermionic Green's function. For the generalized Weyl Hamiltonian, $j_z \sim v_z$, while in the transverse direction

$$j_\perp \sim \frac{\partial}{\partial k_\perp}\big(A_n k_\perp^n\big) \sim A_n k_\perp^{n-1}. \tag{9.29}$$

At frequency $\omega$ we have $k_\perp \sim (\omega/A_n)^{1/n}$, so the typical matrix elements scale as

$$j_z \sim v_z(\omega), \qquad j_\perp \sim A_n(\omega)^{1/n}\, \omega^{(n-1)/n}. \tag{9.30}$$

Invoking the RG-improved replacements $A_n \to A_n(\omega)$, $v_z \to v_z(\omega)$ together with the wave-function factor $Z_\psi(\omega)$ in Eq. (9.13), one obtains (up to nonuniversal prefactors)

$$\sigma_\perp(\omega) \sim \omega\, \frac{Z_\psi^2(\omega)}{v_z(\omega)} \sim \omega\, L_\omega^{-p_\perp}, \tag{9.31}$$

$$\sigma_{zz}(\omega) \sim \omega^{2/n-1}\, Z_\psi^2(\omega)\, \frac{v_z(\omega)}{A_n(\omega)^{2/n}} \sim \omega^{2/n-1}\, L_\omega^{-p_z}, \tag{9.32}$$

with

$$L_\omega \equiv 1 + \bar{\delta}_{12}\alpha_{_N}^{(0)} \ln\frac{\Lambda}{\omega}, \tag{9.33}$$

and exponents

$$p_\perp = 2\eta_\psi + \eta_v \text{ and } p_z = 2\eta_\psi + \frac{2}{n}\,\eta_A - \eta_v. \tag{9.34}$$

Equations (9.31)–(9.34) make the logarithmic scaling explicit and connect it directly to the marginally irrelevant running of $\alpha_{_N}$ and the renormalized parameters $Z_\psi$, $A_n$, and $v_z$.

## 9.6 Effective anomalous dimension $\eta_{\psi,\mathrm{eff}}(E)$

The fermionic field renormalization is determined by the RG equation

$$\frac{d\ln Z_\psi}{d\ell} = -\gamma_0(\ell), \qquad \ell \equiv \ln\frac{\Lambda}{E}, \tag{9.35}$$

where $\gamma_0(\ell)$ is the frequency-projection anomalous dimension (defined via the $ik_0$ component of the one-loop self-energy).

In the infrared for $n > 1$ the Coulomb coupling is marginally irrelevant, as given by Eq. (9.10), and the fermionic anomalous dimension is linear in the running coupling,

$$\gamma_0(\ell) \simeq \frac{\bar{\gamma}_0}{N}\,\alpha_{_N}(\ell), \tag{9.36}$$

where $\bar{\gamma}_0$ is a dimensionless number fixed by the one-loop self-energy integral evaluated with the dressed Coulomb propagator, with the values given in Table 1.

**Multiplicative logarithmic correction for $Z_\psi$.** Substituting Eqs. (9.10) and (9.36) into (9.35) and integrating, we find

$$\begin{aligned}\ln Z_\psi(\ell) &= -\int_0^\ell d\ell'\,\gamma_0(\ell') \simeq -\frac{f_0^{(n)}}{N}\int_0^\ell d\ell'\,\frac{\alpha_N^0}{1+\bar{\delta}_{12}\alpha_{_N}^0\ell'} \\ &= -\frac{f_0^{(n)}}{\bar{\delta}_{12}N}\,\ln\Big(1+\bar{\delta}_{12}\alpha_{_N}^0\ell\Big).\end{aligned} \tag{9.37}$$

Exponentiating gives the standard RG-improved form,

$$Z_\psi(\ell) = \Big(1+\bar{\delta}_{12}\alpha_{_N}^0\ell\Big)^{-\eta_\psi}, \qquad \eta_\psi \equiv \frac{f_0^{(n)}}{\bar{\delta}_{12}N}. \tag{9.38}$$

In terms of the external scale $E$ (set by $E = \max\{T, |\omega|, E_{\boldsymbol{k}}\}$), we obtain

$$Z_\psi(E) = \Big[1+\bar{\delta}_{12}\alpha_{_N}^0\,\ln(\Lambda/E)\Big]^{-\eta_\psi} \equiv L_E^{-\eta_\psi}, \tag{9.39}$$

with $L_E = 1+\bar{\delta}_{12}\alpha_{_N}^0\,\ln(\Lambda/E)$.

**Effective anomalous dimension.** To quantify how a logarithm can *mimic* a power law over a finite range, it is convenient to define the *effective exponent* as the logarithmic slope of $Z_\psi(E)$,

$$\eta_{\psi,\mathrm{eff}}(E) \equiv -\frac{d\ln Z_\psi(E)}{d\ln E}. \tag{9.40}$$

Using Eq. (9.39), we find

$$\begin{aligned}\eta_{\psi,\mathrm{eff}}(E) &= -\frac{d}{d\ln E}\Big[-\eta_\psi\,\ln L_E\Big] = \eta_\psi\,\frac{1}{L_E}\,\frac{dL_E}{d\ln E} \\ &= \eta_\psi\,\frac{\bar{\delta}_{12}\alpha_{_N}^0}{1+\bar{\delta}_{12}\alpha_{_N}^0\,\ln(\Lambda/E)}.\end{aligned} \tag{9.41}$$

Equivalently,

$$\eta_{\psi,\mathrm{eff}}(E) = \frac{\eta_\psi}{\ln(\Lambda/E) + \big(\bar{\delta}_{12}\alpha_{_N}^0\big)^{-1}}. \tag{9.42}$$

Thus, in the deep infrared where $\ln(\Lambda/E) \gg (\bar{\delta}_{12}\alpha^0_{_N})^{-1}$,

$$\eta_{\psi,\mathrm{eff}}(E) \;\simeq\; \frac{\eta_\psi}{\ln(\Lambda/E)} \;\propto\; \frac{1}{\ln(\Lambda/E)}. \tag{9.43}$$

Over any *finite* energy interval around some reference scale $E_*$, one may linearize $\ln Z_\psi(E)$,

$$\ln Z_\psi(E) \approx \ln Z_\psi(E_*) - \eta_{\psi,\mathrm{eff}}(E_*)\,\ln\frac{E}{E_*}, \tag{9.44}$$

valid for

$$\Big|\ln(E/E_*)\Big| \ll \ln(\Lambda/E_*). \tag{9.45}$$

This implies the local power-law fit

$$Z_\psi(E) \approx Z_\psi(E_*)\left(\frac{E}{E_*}\right)^{\eta_{\psi,\mathrm{eff}}(E_*)}. \tag{9.46}$$

Because $\eta_{\psi,\mathrm{eff}}(E)$ drifts only as $1/\ln(\Lambda/E)$, the logarithmic suppression can be well fit by a power law with a slowly running exponent over experimentally accessible windows.

# References


[1] J. Schwinger, Gauge invariance and mass. ii, Phys. Rev. **128**, 2425 (1962).

[2] B. Roy and V. Juričić, Optical conductivity of an interacting Weyl liquid in the collisionless regime, Phys. Rev. B **96**, 155117 (2017).

[3] H. Isobe and N. Nagaosa, Renormalization group study of electromagnetic interaction in multi-dirac-node systems, Phys. Rev. B **87**, 205138 (2013).

[4] M. Peskin and D. Schroeder, *An introduction to quantum field theory* (CRC Press, London, England, 2019).
